# Supplementary material for: Dissecting Hessian: Understanding Common Structure of Hessian in Neural Networks
Source: arXiv:2010.04261 source file (2022-10-21)
Supplement: Supplementary file 1 [file appendix.tex]

\newpage

\section*{Appendix Roadmap}
\begin{enumerate}
    \item In \cref{sec:appendix_derivation_main}, we provide the detailed derivations of Hessian for fully-connected and convolutional layers.
    \item In \cref{sec:appendix_full_hessian}, we provide detailed description on the approximation of dominating eigenvectors of the full hessian.
    \item In \cref{sec:appendix_eigencomp}, we explain how we compute the eigenvalues and eigenvectors of full and layer-wise Hessian numerically.
    \item In \cref{sec:appendix_exp_setup}, we give the detailed experiment setups, including the datasets, network structures, and the training settings we use.
    \item In \cref{sec:appendix_exp_res}, we provide detailed experimental results that are not fully included in the main text.
    \item In \cref{sec:appendix_explanation}, we provide additional and more general explanations of the phenomena we found.
    \item In \cref{sec:appendix_pac}, we give a detailed description of the PAC-Bayes bound that we optimize and the algorithm we use to optimize the bound.
    \item In \cref{sec:appendix_low_rank}, we provided the complete statement and proof for \cref{thm:gaussian_low_rank}.
    \item In \cref{sec:app_codes}, we give a brief description of the source code.
\end{enumerate}

\section{Detailed Derivations}
\label{sec:appendix_derivation_main}
\subsection{Derivation of Hessian}
\input{Appendix_Sections/derivations}
\subsection{Approximating Weight Hessian of Convolutional Layers}
\input{Appendix_Sections/conv_approximation}
\newpage
\input{Appendix_Sections/full_hessian}
\newpage
\input{Appendix_Sections/hessian_calc}
\input{Appendix_Sections/experiment_setup}
\input{Appendix_Sections/additional_exp}
\newpage
\newpage
\input{Appendix_Sections/additional_explanation}
\newpage
\section{Computing PAC-Bayes Bounds with Hessian Approximation}
\input{Appendix_Sections/pac_bayes}

\newpage

\section{Proofs and experiment for the low rank structure of the output Hessian}
\label{sec:appendix_low_rank}
%\documentclass[12pt]{article}
%\usepackage[margin=1in]{geometry}
%\usepackage{hyperref}
%\usepackage{url}
%\usepackage{microtype}
%\newcommand{\fix}{\marginpar{FIX}}
%\newcommand{\new}{\marginpar{NEW}}
%\input{math_commands}
%\usepackage{tabularx}
%\usepackage{graphicx}
%\usepackage{fullpage}
%\usepackage{cite}
%\usepackage{natbib}
%\usepackage{delarray}
%\usepackage{times}
%\usepackage{subfigure}
%\usepackage{color}
%\usepackage{amssymb}
%\usepackage{amsmath}
%\usepackage{amsthm}
%\usepackage{cleveref}
%\usepackage{mathrsfs}
%\usepackage{tikz}
%\usepackage{xspace}
%\usepackage{enumerate}
%\usepackage{epstopdf}

%\usepackage[ruled, vlined]{algorithm2e}
%\usepackage{algorithm}
%\usepackage{algorithmic}
%\usepackage{multirow}
%\usepackage{nameref}
%\usepackage{booktabs}
%\usepackage{mdframed}
%\usepackage{fmtcount}
%\usepackage{footnote}
%\usepackage{bbm}
%\usepackage{thmtools,thm-restate}
%\declaretheorem{theorem}

%\hypersetup{
%    colorlinks=true,       % false: boxed links; true: colored links
%    linkcolor=black,    %cyan,        % color of internal links
%    citecolor=black,        % color of links to bibliography
%    filecolor=magenta,     % color of file links
%    urlcolor=blue
%}

%\title{Hessian low rank proof}

%\begin{document}

%\maketitle

\subsection{Preliminaries}

\subsubsection{Notations}

We use $[n]$ to denote the set $\{1,\cdots,n\}$, and $\n{M}$ to denote the spectral norm of a matrix $M$. We use $\langle A, B\rangle$ to denote the Frobenius inner product of two matrices $A$ and $B$, namely $\langle A, B\rangle\triangleq\sum_{i,j}A_{i,j}B_{i,j}$. Denote $\tr(M)$ the trace of a matrix $M$ and denote $\textbf{1}_c$ the all-one vector of dimension $c$ (the subscript may be omitted when it's clear from the context). Furthermore, for notation simplicity, we will say ``with probability 1 over $\mW^{(1)}$/$\mW^{(2)}$, event $E$ is true'' to denote
\begin{equation}
    \lim_{n\to\infty}\lim_{d\to \infty}\mathop{\Pr}_{\mW^{(1)}\sim\gN(0,\frac{1}{d}\mI_{nd}), \mW^{(2)}\sim\gN(0,\frac{1}{n}\mI_{cn})}\left[E\right] = 1.
\end{equation}

\subsubsection{Problem Setting}

Consider a two layer fully connected ReLU neural network with input dimension $d$, hidden layer dimension $n$ and output dimension $c$. The network is trained with cross-entropy objective $\gL$. Let $\sigma$ denote the element-wise ReLU activation function which acts as $\sigma(x) = x\cdot\1_{x\geq 0}$.
Let $\mW^{(1)}\in\R^{n\times d}$ and $\mW^{(2)}\in\R^{c\times n}$ denote the weight matrices of the first and second layer respectively. 
%Let $\vb^{(1)}\in\R^{n}$ and $\vb^{(2)}\in\R^{c}$ denote the weight matrices of the first and second layer respectively.

Let the neural network have standard normal input $\rvx\sim \gN(0, \mI_d)$. 
Denoting the output of the first and second layer as $\rvy$ and $\rvz$ respectively, we have $\rvy = \sigma(\mW^{(1)}\rvx)$ and $\rvz = \mW^{(2)}\rvy.$ Let $\rvp=\mbox{softmax}(\rvz)$ denote the softmax output of the network. Let $\rmA:=\diag(\rvp)-\rvp\rvp^T$. From the previous analysis of Hessian, we have the output Hessian of the second layer can be written as $\mM := \E[\rmD\mW^{(2)^T}\rmA\mW^{(2)}\rmD]$, where $\rmD:=\diag(\1_{\rvy\geq 0})$ is the diagonal random matrix representing the activations of ReLU function after the first layer.

In this problem, we look into the state of random Gaussian initialization, in which entries of both matrices are i.i.d. sampled from a standard normal distribution, and then re-scaled such that each row of $\mW^{(1)}$ and $\mW^{(2)}$ has norm 1. When taking $n$ and $d$ to infinity, with the concentration of norm in high-dimensional Gaussian random variables, in this problem we assume that entries of $\mW^{(1)}$ are iid sampled from a zero-mean distribution with variance $1/d$, and entries of $\mW^{(2)}$ are iid sampled from a zero-mean distribution with variance $1/n$. This initialization is standard in training neural networks.

Since our formula for the top eigenspace is going to depend on $\mW^{(2)}$, throughout the section when we take expectation we condition on the value of $\mW^{(1)}$ and $\mW^{(2)}$. The expectation is only taken over the input $\rvx\sim \gN(0, \mI_d)$ (due to concentration taking expectation on $\rvx$ is similar to having many samples from the input distribution). In this case, the output Hessian is defined as:
\begin{equation}
\mM\triangleq\E[\rmD\mW^{(2)T}\rmA\mW^{(2)}\rmD].
\end{equation}
%Output Hessian when $\rmD$ is independent of $\rmA$:
%\begin{equation}
%\mM^*=\frac14\pr{\E\left[\mW^{(2)T}\rmA\mW^{(2)}\right]+\diag(\E[\mW^{(2)T}\rmA\mW^{(2)}])}.
%\end{equation}

\subsection{Main Theorem and Proof Sketch}
\label{proof-sketch}

In this section, we will provide a formal statement of our main theorem and its proof sketch. First, we state our main theorem:
\begin{theorem}
\label{main-thm}

For all $\eps > 0$,
\begin{equation}
    \lim_{n\to\infty}\lim_{d\to \infty}\mathop{\Pr}_{\mW^{(1)}\sim\gN(0,\frac{1}{d}\mI_{nd}), \mW^{(2)}\sim\gN(0,\frac{1}{n}\mI_{cn})}\left[\left(\left.\frac{\lambda_c(\mM)}{\lambda_{c-1}(\mM)}\right|_{\mW^{(1)}, \mW^{(2)}}\right) < \eps\right] = 1.
\end{equation}

Besides, for all $\eps>0$, if we define $S_1$ as the top $c-1$ eigenspace of $\mM$, and $S_2$ as $\gR(\mW)\backslash\{\mW\cdot\textbf{1}\}$ where $\gR(\mW)$ is the row space of $\mW$, then
\begin{equation}
    \lim_{n\to\infty}\lim_{d\to \infty}\mathop{\Pr}_{\mW^{(1)}\sim\gN(0,\frac{1}{d}\mI_{nd}), \mW^{(2)}\sim\gN(0,\frac{1}{n}\mI_{cn})}\left[\Overlap\left(S_1,S_2\right)>1-\eps\right] = 1.
\end{equation}

%With probability 1 over $\mW^{(2)}$, $\mM$ is approximately (at most) rank-(c-1), i.e.,
%\begin{equation}
%    \lim_{n\to\infty}\E_{\mW^{(2)}}\left[\frac{\lambda_c(\mM)}{\lambda_{c-1}(\mM)}\right]=0.
%\end{equation}
\end{theorem}
\begin{proofof}{\cref{main-thm}}

First of all, let us repeat the expression for the output Hessian $\mM$:
\begin{equation}
\mM\triangleq\E[\rmD\mW^{(2)T}\rmA\mW^{(2)}\rmD].
\end{equation}

%The expectation is not easy to compute as we condition on $\mW^{(1)}$ and $\mW^{(2)}$. With this conditioning entries of $\rmD$ and $\rmA$ are not independent. However, we will see that in the limit that we are taking, entries of $\rmD$ and the matrix $\mA$ are not actually correlated. If we assume $\rmD$ is independent of $\rmA$ and entries of $\rmD$ are also independently $0/1$ with probability 1/2, then we get the following formula:

%\begin{equation}
%\mM^*\approx\frac14\pr{\E\left[\mW^{(2)T}\rmA\mW^{(2)}\right]+\diag(\E[\mW^{(2)T}\rmA\mW^{(2)}])}.
%\end{equation}

%Even though this is not completely accurate, later in the proof we will show that this is close to be true in the limit. One of the main difficulty is that of course $\rmA$ is not actually independent of $\rmD$ \--- for example, if $\rmD$ happens to be $1$ whenever the first row of $\mW^{(2)}$ is positive, then the first logit output is going to be much larger than the rest which significantly skews the distribution of $\rmA$. We develop a new technique that only requires conditioning on two variables in the matrix $\rmD$, and show that such a conditioning will not change the distribution of $\rmA$.

In the proof, we will first analyze the properties of $\rmD, \mW^{(2)}, \rmA$ separately:

Firstly, $\rmD$ is a diagonal matrix with $0/1$ entries, and the following lemma shows that its entries are independent when the input dimension tends to infinity.
\begin{restatable}{lemma}{lemmaDindependence}
\label{d-independence}
When $d\to \infty$, with probability 1 over $\mW^{(1)}$, the entries of $\rmD$ are independent.
\end{restatable}
Secondly, since each entry of $\mW^{(2)}$ is sampled i.i.d. from a spherical Gaussian distribution, this matrix enjoys some very nice properties when the network width $n$ goes to infinity. We have the following lemma for $\mW^{(2)}$.
\begin{restatable}{lemma}{lemmaWproperties}
\label{lemma:W-properties}
(informal) When $n$ is large enough, each row of $\mW^{(2)}$ has norm very close to 1, and these rows are nearly orthogonal to each other. Besides, the entries (and the average of the entries) cannot be too large.
\end{restatable}
These properties (along with other useful properties) will be formally stated and proved in \cref{proof-w-properties}.

As for matrix $\rmA$, it's very hard to compute its expectation explicitly because the generation of $\rmA$ involves softmax, but we are able to prove some useful properties of $\E[\rmA]$ as shown in the following lemma.

%Since the expectation is taken with respect to the input $\rvx$, which is independent of the matrix $\mW^{(2)}$, the randomness in the expression of $\mM$ lies in $\rmD$ and $\rmA$. We first consider properties of $\rmA$: 
\begin{restatable}{lemma}{lemmaArankc}
\label{lemma:A-rank-c-1}
$\tilde{\rmA}\triangleq\lim_{n\to\infty}\E[\rmA]$ exist and is rank-$(c-1)$ with probability 1 over $\mW^{(2)}$.
\end{restatable}
This lemma is true because $\rmA$ is positive semi-definite (PSD) and is almost always of rank $(c-1)$. Besides, its null space always contains the all-one vector $\textbf{1}_c$.

Having these properties of these three matrices, we then look at the expression of $\mM$ again to see how to compute this expectation. This expectation is not easy to compute as we condition on $\mW^{(1)}$ and $\mW^{(2)}$. With this conditioning, $\rmD$ and $\rmA$ are correlated and hard to decompose. This is when we need the most important observation in our proof: When the input dimension and the network width tend to infinity, $\rmA$ and $\rmD$ can be considered independent when computing $\mM$. These two matrices are actually not independent even when we take the limit: For example, if $\rmD$ happens to be $1$ whenever the first row of $\mW^{(2)}$ is positive, then the first logit output is going to be much larger than the rest which significantly skews the distribution of $\rmA$. However, since the computation of $\mM$ only contains finite-degree polynomials of $\rmA$ and $\rmD$, we only need a weaker form of independence, i.e., the distribution of $\rmA$ is approximately invariant condition on finite entries of $\rmD$, as shown in the following lemma:

\begin{restatable}{lemma}{lemmaAinvariant}
\label{lemmaAinvariant}
Let $\mathcal{D}_{\rmX}$ denote the distribution of $\rmX$, and $TV(\mathcal{D}_1,\mathcal{D}_2)$ denote the total variation distance between $\mathcal{D}_1$ and $\mathcal{D}_2$. Then $\forall i,j\in[n]$, $\forall\eps>0$
\begin{equation}
    \lim_{n\to\infty}\lim_{d\to \infty}\mathop{\Pr}_{\mW^{(1)}\sim\gN(0,\frac{1}{d}\mI_{nd}), \mW^{(2)}\sim\gN(0,\frac{1}{n}\mI_{cn})}\left[TV(\mathcal{D}_{\rmA},\mathcal{D}_{\rmA|\rmD_{i,i}=\rmD_{j,j}=1})>\eps\right] = 0.
\end{equation}
\end{restatable}

The intuition behind this is that $\rmA$ is uniquely determined by the output of the second layer $\rvz$, where $\rvz=\mW^{(2)}\rvy$ is $c$-dimensional and $\rvy$ is an $n$-dimensional vector. Since $\rmD=\diag(\1_{\rvy\geq 0})$, fixing finite number of entries in $\rmD$ is equivalent to fixing the signs of finite entries of $\rvy$. When $n$ is large enough compare to $c$, only constraining finite entries of $\rvy$ shouldn't change the distribution of $\rvz$ by much. The formal proof of this theorem is given in \cref{proof-a-invariant}.

Having \cref{lemmaAinvariant}, we can equivalently consider $\rmA$ and $\rmD$ as independent matrices. To formalize this, we need the following definition:
\begin{definition}
Let $\rmD'$ be an independent copy of $\rmD$ and also independent of $\rmA$. Define $\mM^*\triangleq\E[\rmD'\mW^{(2)T}\rmA\mW^{(2)}\rmD']$.
\end{definition}
In other words, $\mM^*$ is the matrix which has the same expression as $\mM$ except that we assume $\rmD$ is independent of $\rmA$ in $\mM^*$. Then we know that $\mM$ and $\mM^*$ are essentially the same. Since $\rmD$ is a diagonal matrix with $0/1$ entries, multiplying $\rmD$ at both sides of a matrix is equivalent to independently zero out each row and corresponding column with probability $\frac12$. Thus, the probability of each diagonal entry to be kept is $\frac12$ while for off-diagonal ones it's $\frac14$. Formally, we have
\begin{equation}
\mM^*\approx\frac14\pr{\E\left[\mW^{(2)T}\rmA\mW^{(2)}\right]+\diag(\E[\mW^{(2)T}\rmA\mW^{(2)}])}.
\end{equation}
%\textcolor{red}{Rong: I feel we should have a different notation for this $\mW^*$, we shouldn't write equality. We can keep writing $\approx$ but it's not very accurate.}

We have two terms on the right hand side of this equation: $\mT_1\triangleq\E\left[\mW^{(2)T}\rmA\mW^{(2)}\right]$ and $\mT_2\triangleq\diag(\E[\mW^{(2)T}\rmA\mW^{(2)}])$. We make two observations of these two terms. On the one hand, they have the same trace. This is because the diagonal entries of these two matrices are exactly the same. On the other hand, $\mT_1$ is a low rank matrix but $\mT_2$ is approximately full rank. For $\mT_1$, since the expectation is taken over $\rvx$ only, we know that $\mT_1=\mW^{(2)T}\E\left[\rmA\right]\mW^{(2)}$. Note that $\E[A]$ is a rank $(c-1)$ PSD matrix, so $\mT_1$ is also PSD and has rank at most $(c-1)$. $\mT_2$ is a diagonal matrix, and each diagonal entry equals a quadratic form $\vw^{(2)T}_i\E[A]\vw^{(2)}_i$ where $\vw^{(2)}_i$ is the $i$-th column of $\mW^{(2)}$ $(i\in[n])$. This term is always positive unless $\vw^{(2)}_i$ lies in the span of $\textbf{1}_c$, which happens with probability 0. Actually, due to the random nature of $\vw^{(2)}_i$'s, the diagonal terms in $\mT_2$ do not differ too much from one another.

To summarize, $\mT_1$ and $\mT_2$ are both PSD matrices with the same trace, while $\mT_1$ is low-rank but $\mT_2$ is approximately full rank. This intuitively indicates that the positive eigenvalues of $\mT_1$ is significantly large than those of $\mT_2$, making the positive eigenvalues of $\mT_1$ the dominating eigenvalues of $M^*$ and those of $\mT_2$ the thin but long tail of $M^*$'s eigenvalue spectrum.

Now we have know that $\mT_1$ is almost the only contributing term to the top eigenvalues and eigenspaces of $M^*$, so we only need to analyze these for $\mT_1=\mW^{(2)T}\E\left[\rmA\right]\mW^{(2)}$. Since the rows of $\mW^{(2)}$ are close to rank 1 and almost mutually orthogonal, the matrix $\mT_1$ will roughly keeps all the eigenvalues of $\E[A]$, and the top $(c-1)$ eigenspace should roughly be the ``$\mW^{(2)}$-rotated'' version of $\R^c\backslash\{\textbf{1}_c\}$, i.e., $\gR(\mW^{(2)})\backslash\{\mW^{(2)}\cdot\textbf{1}_c\}$.

Despite the arguments above, we have some technical difficulties, the biggest of which is that the dimensions of $\mM$ and $\mM^*$ will become infinite when $n$ goes to infinity. To tackle this problem, we introduce an indirect and more complicated way to do the proof. We first project these matrices onto the row span of $\mW^{(2)}$ and show that this projection roughly keeps all the information of these matrices. Formally, we have the following lemma:
\begin{restatable}{lemma}{lemmaProjPreserveNorm}
\label{corr:proj-preserve-F-norm} With probability 1 over $\mW^{(2)}$,
\[\lim_{n\to\infty}\frac{\fns{\mW\mM\mW^T}}{\fns{\mM}}=1.\]
\end{restatable}
After that, we do the analysis in this finite-dimensional span and finish the proof of our main theorem.

\end{proofof}

\subsection{Detailed Proof}
\label{detailed-proof}

\subsubsection{Proof of \cref{d-independence}}
\label{proof-d-independence}
We first restate \cref{d-independence} here:
\lemmaDindependence*
\begin{proofof}{\cref{d-independence}}
Remember that $\rmD:=\diag(\1_{\rvy\geq 0})$. The off-diagonal entries of $\rmD$ are always 0 and independent of anything. For the diagonal entries, each diagonal entry is decided by a corresponding entry of $\rvy$. Therefore, we only need to prove that the entries of $\rvy$ are independent, and we have the following lemma:
\begin{lemma}
\label{y-independence}
When $d\to \infty$, with probability 1 over $\mW^{(1)}$, the entries of $\rvy$ are independent.
\end{lemma}
\begin{proofof}{\cref{y-independence}}
We will prove this lemma using the multivariate Lindeberg-Feller CLT.
For each $i\in[n]$, let $\vw_i\in\R^d$ denote the $i$-th column vector of $\mW^{(1)}$. Let 
$\rvu_i = \vw_i\ervx_i$,\
then we have \begin{equation}
    \rvu = \sum_{i=1}^d\rvu_i=\sum_{i=1}^d\vw_i\ervx_i = \mW^{(1)}\rvx
\end{equation}
Note that $\ervx_i$'s are i.i.d standard Gaussian. It has the moments:
\begin{equation}
    \E[\ervx_i] = 0,\qquad \E[(\ervx_i - \E[\ervx_i])^2] = 1,\qquad \E[(\ervx_i - \E[\ervx_i])^4] = 3.
\end{equation}
It follows that 
\begin{equation}
   \Var[\rvu_i] = \Var[\vw_i\ervx_i] = \vw_i\vw_i^T.
\end{equation}
Let $\mV = \sum_{i=1}^n Var[\rvu_i]$,
\begin{equation}
    \mV = \sum_{i=1}^d\vw_i\vw_i^T = \mW^{(1)}\mW^{(1)T}.
\end{equation}
As $d\to\infty$, from \cref{lemma:WW-identity} (we replace $n$, $\mW$ with $d$ and $\mW^{(1)}$) we have $\mW^{(1)}\mW^{(1)T}\to \mI_n$ in probability, therefore $\lim_{d\to\infty}\mV = \mI_n$.

We now verify the Lindeberg condition of independent random vectors $\{\rvu_1,\ldots, \rvu_n\}$.
First observe that the fourth moments of the $\rvu_i$ are sufficiently small.
\begin{equation}
\begin{split}
    \lim_{d\to\infty}\sum_{i=1}^d\E\left[\left\Vert\rvu_i\right\Vert^3\right] &= \lim_{d\to\infty}\sum_{i=1}^d\E\left[\left(\sum_{j=1}^n \left(\mW^{(1)}_{ji}\ervx_i\right)^2\right)^2\right]\\
    & \leq\lim_{d\to\infty} \sum_{i=1}^d\E\left[n^2\left(\left(\max_{j\in[n]}\mW^{(2)}_{ji}\right)^2\ervx_i^2\right)^2\right]\\
    & \leq\lim_{d\to\infty} n^2\left(\max_{i\in[d],j\in[n]}\mW^{(2)}_{ji}\right)^4\sum_{i=1}^n\E\left[\left(\ervx_i - \E[\ervx_i]\right)^4\right]
\end{split}
\end{equation}
Since $\E[(\ervx_i - \E[\ervx_i])^4] = 3$ and $\max_{i\in[d],j\in[n]}|\mW^{(2)}_{ji}| < 2d^{-\frac13}$ with probability 1 from \cref{w-not-too-large}, it follows from above that
\begin{equation}
\begin{split}
    \lim_{d\to\infty}\sum_{i=1}^d\E\left[\left\Vert\rvu_i\right\Vert^4\right] \leq n^2\lim_{d\to\infty}\left(2d^{-\frac13}\right)^4\sum_{i=1}^d 3 = 48n^2 \lim_{d\to\infty}d^{-\frac43}d =  48n^2 \lim_{d\to\infty}d^{-\frac13} =0.
\end{split}
\end{equation}
For any $\epsilon > 0$, since $\left\Vert\rvu_{i}\right\Vert > \epsilon$ in the domain of integration,
\begin{equation}
\begin{split}
\lim_{d\to\infty}\sum_{i=1}^d\E\left[\left\Vert\rvu_i\right\Vert^2\textbf{1}\left[\left\Vert\rvu_{i}\right\Vert > \epsilon\right]\right] & < \lim_{d\to\infty}\sum_{i=1}^d\E\left[\frac{\left\Vert\rvu_i\right\Vert^2}{\epsilon^2}\left\Vert\rvu_i\right\Vert^2\textbf{1}\left[\left\Vert\rvu_{i}\right\Vert > \epsilon\right]\right]\\
&\leq \frac{1}{\epsilon^2}\lim_{d\to\infty}\sum_{i=1}^n\E\left[\left\Vert\rvu_i\right\Vert^4\right] = 0.
\end{split}
\end{equation}
As the Lindeberg Condition is satisfied, with $\lim_{n\to\infty}\mV = \mI_c$ in probability we have
\begin{equation}
   \lim_{d\to\infty}\rvu= \lim_{d\to\infty}\sum_{i=1}^d\rvu_i\xrightarrow{D}\gN\left(0,\mI_n\right).
\end{equation}
Thus, since $\rvu$ converges to $\gN\left(0,\mI_n\right)$ in distribution with probability 1 over $\mW^{(1)}$, entries of $\rvu$ are independent. Since $\rvy = \sigma(\rvu)$ and ReLu is an entry-wise operator, entries of $\rvy$ are independent.
\end{proofof}
Since the diagonal entries of $\rmD$ are uniquely determined by the corresponding entries of $\rvy$, we know that when $d\to\infty$, with probability 1 over $\mW^{(1)}$, the entries of $\rmD$ are independent. This finishes the proof of \cref{d-independence}.
\end{proofof}

\subsubsection{Proof of \cref{lemma:W-properties}}
\label{proof-w-properties}
We first restate \cref{lemma:W-properties} here:
\lemmaWproperties*
This is not a formal lemma and will act as the intuition behind the properties of $\mW^{(2)}$. In this section, we will formally state the properties we need and prove them. Besides, for simplicity of notations, we use $\mW$ to denote $\mW^{(2)}$ from now on unless otherwise stated.

\begin{lemma}
\label{lemma:W-expectation}
 For all $i\in[c]$, for all $\eps>0$, $\lim_{n\to\infty}\Pr\pr{\left|\sum_{j=1}^n\mW_{ij}\right|\geq\eps}=0$.
\end{lemma}
\begin{proofof}{\cref{lemma:W-expectation}}
Since each entry of $\mW$ is initialized independently from $\gN(0,\frac1n)$, by Central Limit Theorem we have $\sum_{j=1}^n\mW_{ij}\sim \gN(0,\frac{1}{n})$. For any $\epsilon > 0$, fix $\eps$. By chebyshev's inequality,
\begin{equation}
    \lim_{n\to\infty}\PR\pr{\left|\sum_{j=1}^n\mW_{ij}\right|\geq\epsilon} < \lim_{n\to\infty}\frac{1}{n\eps^2} = 0. 
\end{equation}
\end{proofof}

\begin{lemma}
\label{lemma:W-norm}
For all $\eps>0$, $\lim_{n\to\infty}\Pr\pr{|\fns{\mW}-c|\geq\eps}=0$.\\Besides, for all $i\in[c], \lim_{n\to\infty}\Pr\pr{|\ns{\mW_i}-1|\geq\eps}=0$.
\end{lemma}
\begin{proofof}{\cref{lemma:W-norm}}
Since each entry of $\mW$ is initialized independently from $\gN(0,\frac1n)$, we know that $n\fns{\mW}=\sum_{i=1}^c\sum_{j=1}^nn\mW_{i,j}^2$ follows a $\chi_{cn}^2$-distribution. Using the tail bound provided by Lemma 1 in \cite{laurent2000adaptive}, we know that for large enough $n$,
\begin{equation}
\Pr\pr{|n\fns{\mW}-cn|\geq n\eps}\geq\Pr\pr{|n\fns{\mW}-cn|\geq 2\sqrt{c}n^{3/4}+2n^{1/2}}\leq 2\exp(-n^{1/2}).
\end{equation}
In other words,
\begin{equation}
\lim_{n\to\infty}\Pr\pr{|\fns{\mW}-c|\geq\eps} = \lim_{n\to\infty}\Pr\pr{|n\fns{\mW}-cn|\geq n\eps} = 0.
\end{equation}
Similarly, $\forall i\in[c]$, $n\fns{\mW_i}$ follows a $\chi_n^2$-distribution, so for large enough $n$,
\begin{equation}
\Pr\pr{|n\fns{\mW_i}-n|\geq n\eps}\leq\Pr\pr{|n\fns{\mW}-n|\geq 2n^{3/4}+2n^{1/2}}\leq 2\exp(-n^{1/2}),
\end{equation}
which indicates that
\begin{equation}
\lim_{n\to\infty}\Pr\pr{|\ns{\mW_i}-1|\geq\eps} = \lim_{n\to\infty}\Pr\pr{|n\ns{\mW_i}-n|\geq n\eps} = 0.
\end{equation}
\end{proofof}

\begin{lemma}
\label{lemma:WW-identity}
For all $\eps>0$, $\lim_{n\to\infty}\Pr\pr{\n{\mW\mW^T-\mI_c}\geq\eps}=0$.\\Besides, for all $i,j\in[c], \lim_{n\to\infty}\Pr\pr{|(\mW\mW^T)_{i,j}-\delta_{i,j}|\geq\eps}=0$. Here $\delta$ is the Kronecker delta function, i.e., $\delta_{i,j} = \1_{[i=j]}$.
\end{lemma}
\begin{proofof}{\cref{lemma:WW-identity}}
Since each entry of $\mW$ is initialized independently from $\gN(0,\frac1n)$, we know that $\mW\mW^T$ follows Wishart distribution $\mW_c(\frac1n \mI_c,n)$. Using the third tail bound in Theorem 1 of \cite{zhu2012short}, for large enough $n$, we get
\begin{equation}
\begin{split}
\Pr\pr{\n{\mW\mW^T-\mI_c}\geq\eps} &=\Pr\pr{\n{\frac1n\mW\mW^T-\frac1n\mI_c}\geq\frac{\eps}{n}}\\
&\leq \Pr\pr{\n{\frac1n\mW\mW^T-\frac1n\mI_c}\geq\frac1n\pr{\sqrt{2(c+1)}n^{-1/4}+2cn^{-1/2}}}\\
&\leq 2c\exp(-\sqrt{n}).
\end{split}
\end{equation}
Therefore,
\begin{equation}
\forall\eps>0, \lim_{n\to\infty}\Pr\pr{\n{\mW\mW^T-\mI_c}\geq\eps}=0.
\end{equation}
Moreover, for all $i,j\in[c]$, we have
\begin{equation}
\begin{split}
\Pr\pr{|(\mW\mW^T)_{i,j}-\delta_{i,j}|\geq\eps} &\leq\Pr\pr{\sum_{i,j=1}^c\pr{(\mW\mW^T)_{i,j}-\delta_{i,j}}^2\geq\eps^2}\\
&=\Pr\pr{\fns{\mW\mW^T-\mI_c}\geq\eps^2}\\
&=\Pr\pr{\n{\mW\mW^T-\mI_c}\geq\frac{\eps}{\sqrt{c}}},
\end{split}
\end{equation}
which implies that for all $i,j\in[c]$,
\begin{equation}
\lim_{n\to\infty}\Pr\pr{|(\mW\mW^T)_{i,j}-\delta_{i,j}|\geq\eps}=0.
\end{equation}
\end{proofof}

\begin{lemma}
\label{W-projection}
Let $P_\mW$ be the projection matrix onto the row span of $\mW$, then for all $\eps>0$,
\begin{equation}
    \lim_{n\to\infty}\Pr\left[\fns{\mW^T\mW-P_\mW}>\eps\right]=0.
\end{equation}
\end{lemma}
\begin{proofof}{\cref{W-projection}}
Without loss of generality, we assume that $\eps<1$. Let $\mW_i(i\in[c])$ be the $i$-th row of $\mW$, and we will do the Gram–Schmidt process for the rows of $\mW$. Specifically, the Gram–Schmidt process is as following: Assume that $\{\overline{\mW}_i\}_{i=1}^k$ are the already normalized basis, we set $\mW_{k+1}'\triangleq \mW_{k+1} - \sum_{i=1}^k\langle \mW_{k+1}, \overline{\mW}_i\rangle$ and $\overline{\mW}_{k+1}\triangleq\frac{\mW_{k+1}'}{\n{\mW_{k+1}'}}$. Finally, from the definition of projection matrix, we know that $P_\mW=\overline{\mW}^T\overline{\mW}$.

Let $\eps'\triangleq \frac{\eps^2}{c^3\cdot 16^{2c+1}}$, from \cref{lemma:WW-identity} we know that $\forall i,j\in[c], \lim_{n\to\infty}\Pr\pr{|\mW_i\mW_j^T-\delta_{i,j}|\geq\eps'}=0$. Besides, from \cref{lemma:W-norm} we know that
$\forall i\in[c], \lim_{n\to\infty}\Pr\pr{|\ns{\mW_i}-1|\geq\eps}=0$. Then we use induction to bound the difference between $\mW$ and $\overline{\mW}$. Specifically, we will show that $\forall i\in[c], \n{\overline{\mW}_i-\mW_i}\leq 8^{i}\eps'$. For notation simplicity, in the following proof we will not repeat the probability argument and assume that $\forall i,j\in[c], |\mW_i\mW_j^T-\delta_{i,j}|\leq\eps'$ and $\forall i\in[c], |\ns{\mW_i}-1|\leq\eps'$. We will only use these inequalities finite times so applying a union bound will give the probability result.

For $i=1$, we know that $\overline{\mW}_1 = \frac{\mW_1}{\n{\mW_1}}$ and $|\n{\mW_1}-1|\leq\eps'$, so $\n{\overline{\mW}_i-\mW_i}\leq \eps'$.

If our inductive hypothesis holds for $i\leq k$, then for $i=k+1$, we have 
\begin{equation}\begin{split}
    \forall j\leq k, |\langle \mW_i, \overline{\mW}_j\rangle|&\leq |\langle \mW_i, \mW_j\rangle| + |\langle \mW_i, \overline{\mW}_j-\mW_j\rangle|\\
                                                         &\leq \eps'+ \n{\mW_i}\cdot\n{\overline{\mW}_j-\mW_j}\\
                                                         &\leq \eps'+ (1+\eps')8^j\eps'\\
                                                         &\leq (2^{3j+1}+1)\eps'.
\end{split}\end{equation}
Therefore,
\begin{equation}
    \n{\mW_i'-\mW_i}\leq \sum_{j\in[k]} |\langle \mW_i, \overline{\mW}_j\rangle|\leq \eps'+\sum_{j\in[k]}(2^{3j+1}+1)\eps'\leq (2^{3k+2} - 1)\eps',
\end{equation}
and
\begin{equation}
    |\n{\mW_i'}-1|\leq |\n{\mW_i}-1| + \n{\mW_i'-\mW_i}\leq 2^{3k+2}\eps'.
\end{equation}
Thus,
\begin{equation}\begin{split}
    \n{\overline{\mW}_i-\mW_i}&\leq \n{\overline{\mW}_i-\mW_i'} + \n{\mW_i'-\mW_i}\\
                          &\leq |\n{\mW_i'}-1| + \n{\mW_i'-\mW_i}\\
                          &\leq 8^{k+1}\eps',
\end{split}\end{equation}
which finishes the induction and implies that $\forall \eps>0, \forall i\in[c], \n{\overline{\mW}_i-\mW_i}\leq 8^{i}\eps'$. Thus,
\begin{equation}
\label{eqn:W-equal-W-bar}
    \fns{\overline{\mW}-\mW} = \sum_{i\in[c]} \ns{\overline{\mW}_i-\mW_i}\leq c\cdot 16^c\eps'.
\end{equation}
This means that
\begin{equation}\begin{split}
    \fn{\mW^T\mW-P_\mW} &= \fn{\mW^T\mW-\overline{\mW}^T\overline{\mW}}\\
                  &\leq 2\fn{\mW-\overline{\mW}}\fn{\overline{\mW}} + \fns{\mW-\overline{\mW}}\\
                  &\leq 2c\cdot\sqrt{c}\cdot 8^c\sqrt{\eps'} + c\cdot 16^c\eps'\leq \eps.
\end{split}\end{equation}

\end{proofof}

\begin{lemma}
\label{w-not-too-large}
The largest entry of $\mW^{(2)}$ is reasonably small with high probability as $n$ goes to infinity, namely,
\begin{equation}
\lim_{n\to\infty}\PR\left[\max_{i\in[c],j\in[n]}\left|\mW^{(2)}_{ij}\right\vert > 2n^{-\frac13}\right] = 0
\end{equation}
\end{lemma}

\begin{proofof}{\cref{w-not-too-large}}
For i.i.d. random variables $\rvx_1,\cdots, \rvx_n\sim \gN(0,1)$,
by concentration inequality on maximum of Gaussian random variables, for any $t>0$, we have
\begin{equation}
    \PR\left[\max_{i=1}^n\rvx_i > \sqrt{2\log (2n)} + t\right] < 2e^{-\frac{t^2}{2}}.
\end{equation}
For any $i,j$, since $\mW^{(2)}_{ij}$ are i.i.d. sampled from $\gN(0,\frac1n)$, with rescaling of $1/\sqrt{n}$ we may substitute $\rvx_j$ with $\mW^{(2)}_{ij}$. It follows that
\begin{equation}
    \PR\left[\max_{i\in[c],j\in[n]}\mW^{(2)}_{ij} > \frac{\sqrt{2\log (2cn)} + t}{\sqrt{n}}\right] < 2e^{-\frac{t^2}{2}}.
\end{equation}
Taking $t=n^{\frac16}$, with $c$ as constant, for large $n$ we have $\sqrt{2\log (2cn)} < n^{\frac16}$. Thus for large $n$,
\begin{equation}
\begin{split}
    \PR\left[\max_{i\in[c],j\in[n]}\mW^{(2)}_{ij} > 2n^{-\frac13}\right] &= \PR\left[\max_{i\in[c],j\in[n]}\mW^{(2)}_{ij} > \frac{n^{\frac16} + n^{\frac16}}{\sqrt{n}}\right]\\
    & < \PR\left[\max_{i\in[c],j\in[n]}\mW^{(2)}_{ij} > \frac{\sqrt{2\log (2n)} + n^{\frac16}}{\sqrt{n}}\right] < 2e^{-\frac{n^{\frac13}}{2}}.
\end{split}
\end{equation}
With the same argument, we have
\begin{equation}
    \PR\left[\min_{i\in[c],j\in[n]}\mW^{(2)}_{ij} < -2n^{-\frac13}\right] < 2e^{-\frac{n^{\frac13}}{2}}.
\end{equation}
Passing $n$ to infinity completes the proof.
\end{proofof}

\subsubsection{Proof of \cref{lemma:A-rank-c-1}}
\label{proof-a-rank-c-1}
We first restate \cref{lemma:A-rank-c-1} here:
\lemmaArankc*
Before proving \cref{lemma:A-rank-c-1}, we need some knowledge about the distribution of $\rmA$. Since $\rmA$ is determined by the vector $\rvz$, it suffice to know the distribution of $\rvz$:
\begin{lemma}
\label{z-gaussian}
$\lim_{n\to\infty}\rvz\xrightarrow{d} \gN(0, \frac{\pi-1}{2\pi}\mI_c)$ with probability 1 over $\mW^{(2)}$.
\end{lemma}

\begin{proofof}{\cref{z-gaussian}}
We will prove this lemma using the multivariate Lindeberg-Feller CLT.
For each $i\in[n]$, let $\vw_i\in\R^c$ denote the $i$-th column vector of $\mW^{(2)}$. Let 
$\rvv_i = \vw_i(\ervy_i - \E[\ervy_i])$,
then we have \begin{equation}
\label{eqn:z-expression}
    \rvz = \sum_{i=1}^n\vw_i\ervy_i = \sum_{i=1}^n\rvv_i + \E[\ervy_i]\sum_{i=1}^n\vw_i.
\end{equation}
From \cref{y-independence} we know $\ervy_i$'s are i.i.d. rectified half standard normal. It has the moments:
\begin{equation}
    \E[\ervy_i] = \frac{1}{\sqrt{2\pi}},\qquad \E[(\ervy_i - \E[\ervy_i])^2] = \frac{\pi-1}{2\pi},\qquad \E[(\ervy_i - \E[\ervy_i])^4] = \frac{6\pi^2-10\pi-3}{4\pi^2} < 1.
\end{equation}
It follows that 
\begin{equation}
   Var[\rvv_i] = Var[\vw_i\ervy_i] = \frac{\pi-1}{2\pi}\vw_i\vw_i^T.
\end{equation}
Let $\mV = \sum_{i=1}^n Var[\rvv_i]$,
\begin{equation}
    \mV = \frac{\pi-1}{2\pi}\sum_{i=1}^n\vw_i\vw_i^T = \frac{\pi-1}{2\pi}\mW^{(2)}\mW^{(2)T}.
\end{equation}
As $n\to\infty$, from \cref{lemma:WW-identity} we have $\mW^{(2)}\mW^{(2)T}\to \mI_c$ in probability, therefore $\lim_{n\to\infty}\mV = \frac{\pi-1}{2\pi}\mI_c$.

We now verify the Lindeberg condition of independent random vectors $\{\rvv_1,\ldots, \rvv_n\}$.
First observe that the fourth moments of the $\rvv_i$'s are sufficiently small.
\begin{equation}
\begin{split}
    \lim_{n\to\infty}\sum_{i=1}^n\E\left[\left\Vert\rvv_i\right\Vert^4\right] &= \lim_{n\to\infty}\sum_{i=1}^n\E\left[\left(\sum_{j=1}^c \left(\mW^{(2)}_{ji}\left(\ervy_i - \E[\ervy_i]\right)\right)^2\right)^2\right]\\
    & \leq\lim_{n\to\infty} \sum_{i=1}^n\E\left[c^2\left(\left(\max_{j\in[c]}\mW^{(2)}_{ji}\right)^2\left(\ervy_i - \E[\ervy_i]\right)^2\right)^2\right]\\
    & \leq\lim_{n\to\infty} c^2\left(\max_{i\in[n],j\in[c]}\mW^{(2)}_{ji}\right)^4\sum_{i=1}^n\E\left[\left(\ervy_i - \E[\ervy_i]\right)^4\right].
\end{split}
\end{equation}
Since $\E[(\ervy_i - \E[\ervy_i])^4] < 1$ and $\max_{i\in[n],j\in[c]}|\mW^{(2)}_{ji}| < 2n^{-\frac13}$ with probability 1 from \cref{w-not-too-large}, it follows that
\begin{equation}
\begin{split}
    \lim_{n\to\infty}\sum_{i=1}^n\E\left[\left\Vert\rvv_i\right\Vert^4\right] \leq c^2\lim_{n\to\infty}\left(2n^{-\frac13}\right)^4\sum_{i=1}^n 1 = c^2 \lim_{n\to\infty}16n^{-\frac43}n =  16c^2 \lim_{n\to\infty}n^{-\frac13} =0.
\end{split}
\end{equation}
For any $\epsilon > 0$, since $\left\Vert\rvv_{i}\right\Vert > \epsilon$ in the domain of integration,
\begin{equation}
\begin{split}
\lim_{n\to\infty}\sum_{i=1}^n\E\left[\left\Vert\rvv_i\right\Vert^2\textbf{1}\left[\left\Vert\rvv_{i}\right\Vert > \epsilon\right]\right] & < \lim_{n\to\infty}\sum_{i=1}^n\E\left[\frac{\left\Vert\rvv_i\right\Vert^2}{\epsilon^2}\left\Vert\rvv_i\right\Vert^2\textbf{1}\left[\left\Vert\rvv_{i}\right\Vert > \epsilon\right]\right]\\
&\leq \frac{1}{\epsilon^2}\lim_{n\to\infty}\sum_{i=1}^n\E\left[\left\Vert\rvv_i\right\Vert^4\right] = 0.
\end{split}
\end{equation}
As the Lindeberg Condition is satisfied, with $\lim_{n\to\infty}\mV = \frac{\pi-1}{2\pi}\mI_c$ we have
\begin{equation}
\label{eqn:lemma:sumv-convergence}
    \lim_{n\to\infty}\sum_{i=1}^n\rvv_i\xrightarrow{d}\gN\left(0,\frac{\pi-1}{2\pi}\mI_c\right).
\end{equation}

By \cref{lemma:W-expectation}, we have $\lim_{n\to\infty}\vw_i = \vec0$ with probability 1 over $\mW^{(2)}$, therefore plugging (\cref{eqn:lemma:sumv-convergence}) into (\cref{eqn:z-expression}) we have\begin{equation}
    \lim_{n\to\infty} \rvz\xrightarrow{d}\gN\left(0,\frac{\pi-1}{2\pi}\mI_c\right).
\end{equation}
\end{proofof}
After that, we can proceed to prove \cref{lemma:A-rank-c-1}.

\begin{proofof}{\cref{lemma:A-rank-c-1}}
Note that each entry of $\rmA$ is a quadratic function of $p$, and $p$ is a continuous function of $\rvz$. Therefore, we consider $\rmA$ as a function of $\rvz$ and write $\rmA(\rvz)$ when necessary. From \cref{z-gaussian} we know that $\lim_{n\to\infty}\rvz$ follows a standard normal distribution $\mathcal{N}(0,\alpha \mI_c)$ with probability 1 over $W$, where $\alpha$ is some absolute constant. Therefore, $\tilde{\rmA}\triangleq\lim_{n\to\infty}\E[\rmA]$ exist and it equals $\E[\rmA(\lim_{n\to\infty} \rvz)]=\E_{\rvz\sim\mathcal{N}(0,\alpha \mI_c)}[\rmA(\rvz)]$. For notation simplicity, we will omit the statement ``with probability 1 over $\mW$'' when there is no confusion.

From the definition of $\rmA$ we know that $\rmA\triangleq \text{diag}(p)-pp^T$ where $p$ is the vector obtained by applying softmax to $\rvz$, so $\sum_{i=1}^c p_i=1$ and $\forall i\in[c], p_i\in(0,1)$. Therefore, for any vector $p$ satisfying the previous conditions, we have
\begin{equation}
\textbf{1}^T\rmA\textbf{1} = \sum_{i=1}^c\pr{p_i-\sum_{j=1}^cp_ip_j} = \sum_{i=1}^c(p_i-p_i) =0,
\end{equation}
where $\textbf{1}$ is the all-one vector. Therefore, we know that $\rmA$ has an eigenvalue 0 with eigenvector $\frac{1}{\sqrt{c}}\textbf{1}$. This means that $\E[\rmA]$ also has an eigenvalue 0 with eigenvector $\frac{1}{\sqrt{c}}\textbf{1}$. Thus, $\E[\rmA]$ is at most of rank $(c-1)$.

Then we analyze the other $(c-1)$ eigenvalues of $\tilde{\rmA}$. Since $\rmA=QQ^T$ where $Q=\text{diag}(\sqrt{p})(\mI_c-\textbf{1}p^T)$, we know that $\rmA$ is always a positive semi-definite (PSD) matrix, which indicates that $E[\rmA]$ must also be PSD. Assume the $c$ eigenvalues of $\tilde{\rmA}$ are $\lambda_1\geq\lambda_2\geq\cdots\geq\lambda_{c-1}\geq\lambda_c=0$. Therefore, by definition, we have
\begin{equation}
\lambda_{c-1} = \min_{\vv\in S, \n{\vv}=1}\vv^T\tilde{\rmA}\vv = \E_{\rvz\sim\mathcal{N}(0,\alpha \mI_c)}\left[\min_{\vv\in S, \n{\vv}=1}\vv^T\rmA\vv\right],
\end{equation}
where $S\triangleq\R^c\backslash\gR\{\textbf{1}^T\}$ is the orthogonal subspace of the span of $\textbf{1}$. $\vv\in S$ implies that $\vv\perp\textbf{1}$, i.e., $\sum_{i=1}^c \vv_i = 0$.

Direct computation gives us
\begin{equation}
\vv^T\rmA\vv = \sum_{i=1}^c\vv_i^2p_i-\pr{\sum_{i=1}^c\vv_ip_i}^2.
\end{equation}
Define two vectors $\va,b\in\R^c$ as $\forall i\in[c], \va_i\triangleq \vv_i\sqrt{p_i}, \vb_i\triangleq\sqrt{p_i}$, then $\ns{\vb}=\sum_{i=1}^cp_i=1$ and
\begin{equation}
\vv^T\rmA\vv = \ns{\va}-\langle\va,\vb\rangle^2 = \ns{\va}\cdot\ns{\vb}-\langle \va,\vb\rangle^2.
\end{equation}
Therefore,
\begin{equation}
\vv^T\rmA\vv \geq \ns{\va}\ns{\vb}\sin^2\theta(\va,\vb),
\end{equation}
where $\theta(\va,b)$ is the angle between $\va$ and $\vb$, i.e., $\theta(\va,\vb)\triangleq\arccos\frac{\langle \va,\vb\rangle}{\n{\va}\n{\vb}}$.
Define $p_0\triangleq\min_{i\in[c]}p_i$, then
\begin{equation}
\ns{\va} = \sum_{i=1}^c\vv_i^2p_i \geq \sum_{i=1}^c\vv_i^2p_0 = p_0\ns{\vv} = p_0.
\end{equation}
Since $\n{\vb}=1$, we have
\begin{equation}
\sin^2\theta(\va,\vb) = \frac{\ns{\va-\langle \va,\vb\rangle\cdot \vb}}{\ns{\va}}.
\end{equation}
Besides,
\begin{equation}\begin{split}
\ns{\va-\langle \va,\vb\rangle\cdot \vb} &= \sum_{i=1}^c\pr{\vv_i\sqrt{p_i}-\pr{\sum_{j=1}^c\vv_jp_j}\sqrt{p_i}}^2\\
                                 &= \sum_{i=1}^cp_i\pr{\vv_i-\sum_{j=1}^c\vv_jp_j}^2\\
                                 &\geq p_0\sum_{i=1}^c\pr{\vv_i-\sum_{j=1}^c\vv_jp_j}^2.
\end{split}\end{equation}
Define $s\triangleq\arg\max_{i\in[c]}{\vv_i}$ and $t\triangleq\arg\min_{i\in[c]}{\vv_i}$, then
\begin{equation}
\sum_{i=1}^c\pr{\vv_i-\sum_{j=1}^c\vv_jp_j}^2\geq \pr{\vv_s-\sum_{j=1}^c\vv_jp_j}^2 + \pr{\vv_t-\sum_{j=1}^c\vv_jp_j}^2 \geq \frac{(\vv_s-\vv_t)^2}{2}.
\end{equation}
From $\n{\vv}=1$ we know that $\max_{i\in[c]}|\vv_i|\geq\frac{1}{\sqrt{c}}$. Besides, since $\sum_{i=1}^c\vv_i=0$, we have $\vv_s>0>\vv_t$. Therefore, $\vv_s-\vv_t>\max_{i\in[c]}|\vv_i|\geq\frac{1}{\sqrt{c}}$. As a result,
\begin{equation}
\ns{\va-\langle \va,\vb\rangle\cdot \vb} \geq p_0\cdot \frac{(\vv_s-\vv_t)^2}{2} > \frac{p_0}{2c}.
\end{equation}
Moreover,
\begin{equation}
\ns{\va} = \sum_{i=1}^c \vv_i^2p_i \leq \sum_{i=1}^c p_i = 1.
\end{equation}
Thus,
\begin{equation}
\sin^2\theta(\va,\vb) \geq \frac{\frac{p_0}{2c}}{1} = \frac{p_0}{2c},
\end{equation}
which means that
\begin{equation}
\vv^T\rmA\vv \geq p_0\cdot 1\cdot\frac{p_0}{2c} = \frac{p_0^2}{2c}.
\end{equation}
Now we analyze the distribution of $p_0$. Since $\rvz$ follows a spherical Gaussian distribution $\mathcal{N}(0,\alpha \mI_c)$, we know that the entries of $\rvz$ are totally independent. Besides, for each entry $\rvz_i(i\in[c])$, we have $|\rvz_i|<\alpha$ with probability $\beta$, where $\beta\approx 0.68$ is an absolute constant. Therefore, with probability $\beta^c$, forall entries $\rvz_i(i\in[c])$, we have $|\rvz_i|<\alpha$. In this case,
\begin{equation}
p_0 = \frac{\exp(\min_{i\in[c]}\rvz_i)}{\sum_{i=1}^c\exp(\rvz_i)}\geq\frac{\exp(-\alpha)}{c\exp(\alpha)}.
\end{equation}
In other cases, we know that $p_0>0$. Thus,
\begin{equation}
\label{lower-bound-c-1-eigenvalue-of-A}
\lambda_{c-1} = \E_{\rvz\sim\mathcal{N}(0,\alpha \mI_c)}\left[\min_{\vv\in S, \n{v}=1}\vv^T\rmA\vv\right]\geq \beta^c\cdot\frac{\pr{\frac{\exp(-\alpha)}{c\exp(\alpha)}}^2}{2c}.
\end{equation}
The right hand side is independent of $n$. Therefore, $\lambda_{c-1}>0$, which means that $\tilde{\rmA}$ has exactly $(c-1)$ positive eigenvalues and a $0$ eigenvalue, and the eigenvalue gap between the smallest positive eigenvalue and 0 is independent of $n$.
\end{proofof}

\subsubsection{Proof of \cref{lemmaAinvariant}}
\label{proof-a-invariant}
We first restate \cref{lemmaAinvariant} here:
\lemmaAinvariant*

\begin{proofof}{\cref{lemmaAinvariant}}
The proof of this lemma requires knowledge about the distributions of $\rmA$ condition on two diagonal entries of $\rmD$. Since $\rmA$ can be uniquely determined by $\rvz$, it is enough for us to know the distribution of $\rvz$ condition on the two entries of $\rmD$. We use the following lemma to analyze this:

\begin{lemma}
\label{lemma:z-converge-with-condition}
With probability 1 over $\mW^{(2)}$,  for any $i,j\in[n]$, for any $(p,q)\in\{0,1\}^2$, 
\begin{equation}
\lim_{n\to\infty}P(\rvz\vert D_{ii}=p,D_{jj}=q) \xrightarrow{d}\rvz.
\end{equation}

\end{lemma}
\begin{proofof}{\cref{lemma:z-converge-with-condition}}
With $\{\vw_1,\ldots, \vw_n\}$ and $\{\rvv_1,\ldots, \rvv_n\}$ defined as above, since different summands contributing to $\rvz$ are independent, and every $\rv_i$ is only affected by its corresponding $D_{ii}$,
\begin{equation}
\begin{split}
    P(\rvz\vert D_{ii}=p,D_{jj}=q) &= \rvz - \rvv_i + P(\rvv_i\vert D_{ii}=p) - \rvv_j + P(\rvv_j\vert D_{jj}=q)\\
    &= \rvz - \vw_i(\ervy_i - P(\ervy_i\vert D_{ii}=p)) + \vw_j(\rvy_j - P(\rvy_j\vert D_{jj}=q)).
\end{split}
\end{equation}
For any $i\in[n]$, with the condition of $D_{ii} = p$, when $p=0$, $P(\ervy_i\vert D_{ii}=p)=0$; when conditioned with $p=1$, $P(\ervy_i\vert D_{ii}=p)$ is of a half standard normal distribution truncated at 0. In both cases the conditional distribution of $P(\ervy_i\vert D_{ii}=p)$ and hence $\ervy_i-P(\ervy_i\vert D_{ii}=p)$ has bounded mean and variance. For any $\vw_i$, by \cref{w-not-too-large} we have
\begin{equation}
    \left\Vert\vw_i\right\Vert \leq \sqrt{c\left(\max_{i\in[c],j\in[n]}\mW^{(2)}_{ij}\right)^2} < \sqrt{4cn^{-\frac{2}{3}}} \text{ with probability 1 over }\mW^{(2)}.
\end{equation}
Since $\lim_{n\to\infty}\sqrt{4cn^{-\frac{2}{3}}}=0$, as $n$ goes to infinity we have \begin{equation}
    \vw_i(\ervy_i - P(\ervy_i\vert D_{ii}=p))\xrightarrow{d} 0 \text{ with probability 1 over } \mW^{(2)}.
\end{equation}
Therefore
\begin{equation}
    P(\rvz\vert D_{ii}=p,D_{jj}=q) = \rvz - \vw_i(\ervy_i - P(\ervy_i\vert D_{ii}=p)) + \vw_j(\rvy_j - P(\rvy_j\vert D_{jj}=q)) \xrightarrow{d} \rvz.
\end{equation}
\end{proofof}
From \cref{lemma:z-converge-with-condition} we conclude that
\begin{equation}
    \lim_{n\to\infty}\lim_{d\to \infty}\mathop{\Pr}_{\mW^{(1)}\sim\gN(0,\frac{1}{d}\mI_{nd}), \mW^{(2)}\sim\gN(0,\frac{1}{n}\mI_{cn})}\left[TV(\mathcal{D}_{\rvz},\mathcal{D}_{\rvz|\rmD_{i,i}=\rmD_{j,j}=1})>\eps\right] = 1.
\end{equation}
Since $\rmA$ can be uniquely determined by $\rvz$, we have
\begin{equation}
    TV(\mathcal{D}_{\rvz},\mathcal{D}_{\rvz|\rmD_{i,i}=\rmD_{j,j}=1}) \geq TV(\mathcal{D}_{\rmA},\mathcal{D}_{\rmA|\rmD_{i,i}=\rmD_{j,j}=1}).
\end{equation}
Therefore,
\begin{equation}
    \lim_{n\to\infty}\lim_{d\to \infty}\mathop{\Pr}_{\mW^{(1)}\sim\gN(0,\frac{1}{d}\mI_{nd}), \mW^{(2)}\sim\gN(0,\frac{1}{n}\mI_{cn})}\left[TV(\mathcal{D}_{\rmA},\mathcal{D}_{\rmA|\rmD_{i,i}=\rmD_{j,j}=1})>\eps\right] = 0.
\end{equation}
This finishes the proof of \cref{lemmaAinvariant}.
\end{proofof}

\subsubsection{Proof of \cref{corr:proj-preserve-F-norm}}
\label{proof-proj-preserve-F-norm}
We first restate \cref{corr:proj-preserve-F-norm} here:
\lemmaProjPreserveNorm*
\begin{proofof}{\cref{corr:proj-preserve-F-norm}}
To prove the equivalence between $\fns{\mW\mM\mW^T}$ and $\fns{\mM}$, we need some other terms, including terms containing $\mM^*$, as bridges. To prove the equivalence between $\mM$ and $\mM^*$, we need the following lemma which explains the reason why we only need the weaker sense of independence (\cref{lemmaAinvariant}) instead of the total independence between $\rmA$ and $\rmD$.
\begin{lemma}
\label{lemma:polynomial}
Let $p(\rmA,\rmD)$ be a homogeneous polynomial of $\rmA$ and $\rmD$ and is degree 1 in $\rmA$ and degree 2 in $\rmD$, and let the coefficients in $p$ are upper bounded in $\ell_1$-norm by an absolute constant. Also let $\rmA'$ be an independent copy of $\rmA$. Then
\begin{equation}
    \lim_{n\to\infty}\lim_{d\to \infty}\mathop{\Pr}_{\mW^{(1)}\sim\gN(0,\frac{1}{d}\mI_{nd}), \mW^{(2)}\sim\gN(0,\frac{1}{n}\mI_{cn})}\left[|\E[p(\rmA,\rmD)]-\E[p(\rmA',\rmD)]|>\eps\right] = 0.
\end{equation}
\end{lemma}
\begin{proofof}{\cref{lemma:polynomial}}
Assume that $p(\rmA,\rmD)=\sum_{i=1}^m c_i\rmA_{s(i),t(i)}\rmD_{u(i),u(i)}\rmD_{v(i),v(i)}$, then from linearity of expectation we know
\begin{equation}
    \E[p(\rmA,\rmD)] = \sum_{i=1}^m c_i\E[\rmA_{s(i),t(i)}\rmD_{u(i),u(i)}\rmD_{v(i),v(i)}].
\end{equation}
Since the entries of $\rmD$ can only be $0$ or $1$, we have
\begin{equation}
    \E[\rmA_{s(i),t(i)}\rmD_{u(i),u(i)}\rmD_{v(i),v(i)}] = \E[\rmA_{s(i),t(i)}|\rmD_{u(i),u(i)}=\rmD_{v(i),v(i)}=1].
\end{equation}
Assume that the upper bound of the sum of $|c_i|$s is $\alpha$, i.e., $\sum_{i=1}^m|c_i|\geq \alpha$. Set $\eps'=\frac{\eps}{\alpha}$ and from \cref{lemmaAinvariant} we know that
\begin{equation}
    \lim_{n\to\infty}\lim_{d\to \infty}\mathop{\Pr}_{\mW^{(1)}\sim\gN(0,\frac{1}{d}\mI_{nd}), \mW^{(2)}\sim\gN(0,\frac{1}{n}\mI_{cn})}\left[TV(\mathcal{D}_{\rmA},\mathcal{D}_{\rmA|\rmD_{i,i}=\rmD_{j,j}=1})>\eps'\right] = 0.
\end{equation}
In other words, with probability 1 we have $TV(\mathcal{D}_{\rmA},\mathcal{D}_{\rmA|\rmD_{i,i}=\rmD_{j,j}=1})\leq \eps'$. Besides, since $\forall i,j\in[c], i\neq j, p_i,p_j, p_i+p_j\in(0,1)$, each entry of $A$ (either $p_i-p_i^2$ or $-p_ip_j$) must be in $(-\frac14,\frac14)$. Therefore, when $n$ and $d$ goes to infinity, with probability 1 over $\mW^{(1)}$ and $\mW^{(2)}$ we have
\begin{equation}\begin{split}
    &\|\E[\rmA_{s(i),t(i)}|\rmD_{u(i),u(i)}=\rmD_{v(i),v(i)}=1] - \E[\rmA_{s(i),t(i)}]\|\\
\leq&TV(\mathcal{D}_{\rmA},\mathcal{D}_{\rmA|\rmD_{i,i}=\rmD_{j,j}=1})\cdot\pr{\frac14-\pr{-\frac14}}\leq\frac{\eps'}{2}.
\end{split}\end{equation}
Thus,
\begin{equation}\begin{split}
    |\E[p(\rmA,\rmD)]-\E[p(\rmA',\rmD)]|&\leq\sum_{i=1}^m|c_i|\cdot\|\E[\rmA_{s(i),t(i)}|\rmD_{u(i),u(i)}=\rmD_{v(i),v(i)}=1] - \E[\rmA_{s(i),t(i)}]\|\\
                                        &\leq\pr{\sum_{i=1}^m|c_i|}\cdot \frac{\eps'}{2}\leq\alpha\cdot\frac{\eps}{2\alpha}<\eps.
\end{split}\end{equation}
This finishes the proof of \cref{lemma:polynomial}.
\end{proofof}
After this, using \cref{lemmaAinvariant}, we have the following lemmas:

\begin{lemma}
\label{lemma:M-equivalence} with probability 1 over $\mW$,
\[\lim_{n\to\infty}\frac{\fns{\mM}}{\fns{\mM^*}}=1.\]
\end{lemma}
\begin{proofof}{\cref{lemma:M-equivalence}}
Let $(\rmD',\rmA')$ be an independent copy of $(\rmD,\rmA)$, then
\begin{equation}
\begin{split}
    \fns{\mM} &=\fns{\E[\rmD\mW^T\rmA\mW\rmD]}\\
    &=\E\left[\langle \rmD\mW^T\rmA\mW\rmD,\rmD'\mW^T\rmA'\mW\rmD'\rangle\right]\\
    &=\E\left[\tr\left(\rmD\mW^T\rmA\mW\rmD\rmD'\mW^T\rmA'\mW\rmD'\right)\right]\\
    &=\E\left[\tr\left(\mW\rmD'\rmD\mW^T\rmA\mW\rmD\rmD'\mW^T\rmA'\right)\right].
\end{split}
\end{equation}
Expressing the term inside the expectation as a polynomial of entries of $\rmA$, $\rmD$, $\rmA'$ and $\rmD'$, we get
\begin{equation}
\begin{split}
     &\tr\left(\mW\rmD'\rmD\mW^T\rmA\mW\rmD\rmD'\mW^T\rmA'\rangle\right) \\
    =&\sum_{i=1}^c\left(\mW\rmD'\rmD\mW^T\rmA\mW\rmD\rmD'\mW^T\rmA'\right)_{i,i}\\
    =&\sum_{i,j=1}^c\pr{\mW\rmD'\rmD\mW^T\rmA}_{i,j}\pr{\mW\rmD\rmD'\mW^T\rmA'}_{j,i}\\
    =&\sum_{i,j=1}^c\pr{\sum_{k=1}^c\sum_{l=1}^n\mW_{i,l}\mW_{k,l}\rmD_{l,l}'\rmD_{l,l}\rmA_{k,j}}\pr{\sum_{s=1}^c\sum_{t=1}^n\mW_{j,t}\mW_{s,t}\rmD_{t,t}\rmD_{t,t}'\rmA_{s,i}'}\\
    =&\sum_{i,j,k,s=1}^c\sum_{l,t=1}^n \mW_{i,l}\mW_{k,l}\mW_{j,t}\mW_{s,t}\rmA_{k,j}\rmA_{s,i}'\rmD_{l,l}\rmD_{l,l}'\rmD_{t,t}\rmD_{t,t}'.
\end{split}
\end{equation}
Now we can bound the $\ell_1$ norm of the coefficient of this polynomial as follows (note that absolute value of each entry of $\rmA$ is bounded by 1):
\begin{equation}
\begin{split}
     &\n{\sum_{i,j,k,s=1}^c\sum_{l,t=1}^n \mW_{i,l}\mW_{k,l}\mW_{j,t}\mW_{s,t}}_1\\
    \leq &\sum_{i,j,k,s=1}^c\sum_{l,t=1}^n |\mW_{i,l}|\cdot|\mW_{k,l}|\cdot|\mW_{j,t}|\cdot|\mW_{s,t}|\\
    =    &\pr{\sum_{i,k=1}^c\sum_{l=1}^n|\mW_{i,l}|\cdot|\mW_{k,l}|}\pr{\sum_{j,s=1}^c\sum_{t=1}^n|\mW_{j,t}|\cdot|\mW_{s,t}|}\\
    \leq &\pr{\sum_{i,k=1}^c\sum_{l=1}^n\frac{\mW_{i,l}^2+\mW_{k,l}^2}{2}}\pr{\sum_{j,s=1}^c\sum_{t=1}^n\frac{\mW_{j,t}^2+\mW_{s,t}^2}{2}}\\
    =    &\pr{\sum_{i,k=1}^c\frac{\ns{\mW_i}+\ns{\mW_k}}{2}}\pr{\sum_{j,s=1}^c\frac{\ns{\mW_j}+\ns{\mW_s}}{2}}\\
    =    &(c\fns{\mW})^2=c^2\fn{\mW}^4.
\end{split}
\end{equation}
When $n\to\infty$, we know that $\fn{\mW}^2=O(c)$ with probability 1 over $\mW$, so the coefficient of this polynomial is $\ell_1$-norm bounded. We know from \cref{lemmaAinvariant} that the distribution of $\rmA$ is invariant condition on two entries of $\rmD$. Furthermore, since $\rmA'$ and $\rmD'$ are independent copies of $\rmA$ and $\rmD$, we know that the distribution of $(\rmA,\rmA')$ is invariant conditioning on two entries of $\rmD$ and two entries of $\rmD'$. Each term in this polynomial is a 4-th order term containing two entries from $\rmD$ and two from $\rmD'$. This combined with \cref{lemma:polynomial} gives us
\begin{equation}
    \lim_{n\to\infty}\frac{\fns{\mM}}{\fns{\mM^*}}=1.
\end{equation}

\end{proofof}

\begin{lemma}
\label{lemma:WMW-equivalence}
For all $i,j\in[c], \lim_{n\to\infty}((\mW\mM\mW^T)_{i,j}-(\mW\mM^*\mW^T)_{i,j})=0$. Thus, \[\lim_{n\to\infty}\frac{\fns{\mW\mM\mW^T}}{\fns{\mW\mM^*\mW^T}}=1.\]
\end{lemma}
\begin{proofof}{\cref{lemma:WMW-equivalence}}
This proof is very similar to that of \cref{lemma:M-equivalence}. First, we focus on a single entry of the matrix $\mW\mM\mW^T$ and express it as a polynomial of entries of $\rmD$:
\begin{equation}
\begin{split}
(\mW\mM\mW^T)_{i,j} &= \E[(\mW\rmD\mW^T\rmA\mW\rmD\mW^T)_{i,j}]\\
              &= \E\left[\sum_{k=1}^c(\mW\rmD\mW^T\rmA)_{i,k}(\mW\rmD\mW^T)_{k,j}\right]\\
              &= \E\left[\sum_{k=1}^c\pr{\sum_{s=1}^c\sum_{l=1}^n\mW_{i,l}\mW_{s,l}\rmD_{l,l}\rmA_{s,k}}\pr{\sum_{t=1}^n\mW_{k,j}\mW_{j,t}\rmD_{t,t}}\right]\\
              &= \E\left[\sum_{k,s=1}^c\sum_{l,t=1}^n\rmA_{s,k}\mW_{i,l}\mW_{s,l}\mW_{k,t}\mW_{j,t}\rmD_{l,l}\rmD_{t,t}\right].
\end{split}
\end{equation}
Then we bound the $\ell_1$ norm of the coefficients of this polynomial as follows:
\begin{equation}
\begin{split}
    &\n{\sum_{k,s=1}^c\sum_{l,t=1}^n\rmA_{s,k}\mW_{i,l}\mW_{s,l}\mW_{k,t}\mW_{j,t}}_1\\
    \leq &\sum_{k,s=1}^c\sum_{l,t=1}^n|\mW_{i,l}|\cdot|\mW_{s,l}|\cdot|\mW_{k,t}|\cdot|\mW_{j,t}|\\
    =    &\pr{\sum_{s=1}^c\sum_{l=1}^n|\mW_{i,l}|\cdot|\mW_{s,l}|}\pr{\sum_{k=1}^c\sum_{t=1}^n|\mW_{k,t}|\cdot|\mW_{j,t}|}\\
    \leq &\pr{\sum_{s=1}^c\sum_{l=1}^n\frac{\mW_{i,l}^2+\mW_{s,l}^2}{2}}\pr{\sum_{k=1}^c\sum_{t=1}^n\frac{\mW_{k,t}^2+\mW_{j,t}^2}{2}}\\
    =    &\pr{c\ns{\mW_i}+\fns{\mW}}\pr{c\ns{\mW_j}+\fns{\mW}}\\
    \leq &(2c\fns{\mW})^2=4c^2\fn{\mW}^4.
\end{split}
\end{equation}
Similar to \cref{lemma:M-equivalence}, this coefficient is $\ell_1$-norm bounded. Therefore, using \cref{lemma:polynomial}, we have with probability 1 over $\mW$, for all $i,j\in[c], \lim_{n\to\infty}((\mW\mM\mW^T)_{i,j}-(\mW\mM^*\mW^T)_{i,j})=0$, which indicates that \[\lim_{n\to\infty}\frac{\fns{\mW\mM\mW^T}}{\fns{\mW\mM^*\mW^T}}=1.\]
\end{proofof}

\begin{lemma}
\label{F-norm-equal}
\[\lim_{n\to\infty}\frac{\fns{\mW\mM^*\mW^T}}{\fns{\mM^*}}=1.\]
\end{lemma}
\begin{proofof}{\cref{F-norm-equal}}
The proof of this lemma will be divided into two parts. In the first part, we will estimate the Frobenius norm of $\mM^*$, and in the second part we do the same thing for $\mW\mM^*\mW^T$.

\textbf{Part 1:} We know from the definition of $\mM^*$ that
\begin{equation}
\label{lemma:M-star}
\mM^*=\frac14\pr{\E[\mW^T\rmA\mW]+\diag(\E[\mW^T\rmA\mW])}.
\end{equation}
Define $\tilde{\rmA}:=\E[\rmA]$, then
\begin{equation}
\E[\mW^T\rmA\mW] = \mW^T\E[\rmA]\mW = \mW^T\tilde{\rmA}\mW.
\end{equation}
From \cref{lemma:WW-identity}, $\forall\eps'>0$, with probability 1 we have $\n{\mW\mW^T-I_c}\leq\eps'$. Besides, from \cite{kleinman1968design} we know that for positive semi-definite matrices $A$ and $B$ we have $\lambda_{\min}(A)\tr(B)\leq \tr(AB)\leq \lambda_{\max}(A)\tr(B)$, so
\begin{equation}
\begin{split}
    \bigg|\fns{\mW^T\tilde{\rmA}\mW} - \fns{\tilde{\rmA}}\bigg|
    &=\Big|\tr(\mW^T\tilde{\rmA}\mW\mW^T\tilde{\rmA}\mW)-\tr(\tilde{\rmA}\tilde{\rmA})\Big|\\
    &=\Big|\tr(\mW\mW^T\tilde{\rmA}\mW\mW^T\tilde{\rmA})-\tr(\tilde{\rmA}\tilde{\rmA})\Big|\\
    &\leq\Big|\pr{\n{\mW\mW^T-I_c}+1}\tr(\tilde{\rmA}\mW\mW^T\tilde{\rmA})-\tr(\tilde{\rmA}\tilde{\rmA})\Big|\\
    &=\Big|\pr{\n{\mW\mW^T-I_c}+1}\tr(\mW\mW^T\tilde{\rmA}\tilde{\rmA})-\tr(\tilde{\rmA}\tilde{\rmA})\Big|\\
    &\leq\Big|\pr{\n{\mW\mW^T-I_c}+1}^2\tr(\tilde{\rmA}\tilde{\rmA})-\tr(\tilde{\rmA}\tilde{\rmA})\Big|\\
    &\leq\n{\mW\mW^T-I_c}^2\fns{\tilde{A}} + 2\n{\mW\mW^T-I_c}\fns{\tilde{A}}.
\end{split}
\end{equation}
For any $\eps>0$, set $\eps'=\min\{\frac{\eps}{4},\frac{\sqrt{\eps}}{2}\}$ gives us with probability 1,
\begin{equation}
    \lim_{n\to\infty}\frac{\bigg|\fns{\mW^T\tilde{\rmA}\mW} - \fns{\tilde{\rmA}}\bigg|}{\fns{\tilde{\rmA}}}=0,
\end{equation}
i.e.,
\begin{equation}
    \lim_{n\to\infty}\frac{\fns{\mW^T\tilde{\rmA}\mW}}{\fns{\tilde{\rmA}}}=1.
\end{equation}
Besides, if we denote the $i$-th column of $\mW$ by $\vw_i$, then
\begin{equation}
\begin{split}
\fns{diag(\E[\mW^T\rmA\mW])} &= \sum_{i=1}^n (\vw_i^T\tilde{\rmA}\vw_i)^2\\
                      &\leq \sum_{i=1}^n \pr{\ns{\vw_i}\cdot\n{\tilde{\rmA}}}^2\\
                      &= \ns{\tilde{\rmA}}\sum_{i=1}^n \n{\vw_i}^4.
\end{split}
\end{equation}
Since $\E[n^2\n{\vw_i}^4]=c^2+2c$, by the additive form of Chernoff bound we get
\begin{equation}
\Pr\pr{\sum_{i=1}^n\n{\vw_i}^4\geq \frac{c^2+3c}{n}}=\Pr\pr{\frac{\sum_{i=1}^nn^2\n{\vw_i}^4}{n}-(c^2+2c)\geq c}\leq e^{-2nc^2}.
\end{equation}
Therefore, when $n\to\infty$, with probability 1 we have
\begin{equation}
\fns{\diag(\E[\mW^T\rmA\mW])}\leq \ns{\tilde{\rmA}}\sum_{i=1}^n \n{\vw_i}^4\leq \ns{\tilde{\rmA}}\cdot\frac{c^2+3c}{n}.
\end{equation}
Thus, with probability 1,
\begin{equation}
\label{lemma:W-diag-neg}
\lim_{n\to\infty}\frac{\fns{\diag\left(\E\left[\mW^T\rmA\mW\right]\right)}}{\fns{\mW^T\tilde{\rmA}\mW}} = 0,
\end{equation}
i.e.,
\begin{equation}
\lim_{n\to\infty}\frac{\frac{1}{16}\fns{\tilde{\rmA}}}{\fns{\mM^*}} = 1.
\end{equation}
\textbf{Part 2:} Plug equation \cref{lemma:M-star} into $\mW\mM^*\mW$ and we get
\begin{equation}
\mW\mM^*\mW = \frac14\pr{\E[\mW\mW^T\rmA\mW\mW^T]+\E[\mW \diag(\mW^T\rmA\mW)\mW^T]}.
\end{equation}
Similar to \textbf{Part 1}, when $n\to\infty$, with probability 1, we have
\begin{equation}
\lim_{n\to\infty}\frac{\fns{\E[\mW\mW^T\rmA\mW\mW^T]}}{\fns{\tilde{\rmA}}} = 1.
\end{equation}
Besides, when $n\to\infty$, with probability 1 we have
\begin{equation}
\fns{\mW\diag(\E[\mW^T\rmA\mW])\mW^T}\leq \fns{\mW}\ns{\tilde{\rmA}}\sum_{i=1}^n \n{\vw_i}^4\leq \ns{\tilde{\rmA}}\cdot\frac{c^2+3c}{n}\fns{\mW}.
\end{equation}
As a result, with probability 1,
\begin{equation}
\lim_{n\to\infty}\frac{\fns{\mW\diag(\E[\mW^T\rmA\mW])\mW^T}}{\fns{\mW\mW^T\tilde{\rmA}\mW\mW^T}} = 0,
\end{equation}
i.e.,
\begin{equation}
\lim_{n\to\infty}\frac{\frac{1}{16}\fns{\tilde{\rmA}}}{\fns{\mW\mM^*\mW^T}} = 1.
\end{equation}
Combining the results of \textbf{Part 1} and \textbf{Part 2} proves this lemma.
\end{proofof}
Combining \cref{lemma:M-equivalence}, \cref{lemma:WMW-equivalence}, and \cref{F-norm-equal} directly finishes the proof of \cref{corr:proj-preserve-F-norm}.
\end{proofof}

\subsubsection{Proof of Theorem \cref{main-thm}}
\label{proof-main-thm}

\begin{proofof}{Theorem \cref{main-thm}}
Now we can proceed to the proof of our main theorem. In this proof, we will use the bounds for $\fn{\mM}$, which are formalized into the lemma below:

\begin{lemma}
\label{lemma:M-F-norm-bound}
With probability 1, $\lim_{n\to\infty}\fn{\mM}$ is both lower bounded and upper bounded by constants that are independent of $n$.
\end{lemma}
\begin{proofof}{\cref{lemma:M-F-norm-bound}}
From \cref{lemma:M-equivalence} we know that $\lim_{n\to\infty}\frac{\fn{\mM}}{\fn{\mM^*}}=1$, so we only need to bound $\lim_{n\to\infty}\fn{\mM^*}$. Since $\mM^*=\frac14\pr{\E[\mW^T\rmA\mW]+\text{diag}(\E[\mW^T\rmA\mW])}$ and $\langle\E[\mW^T\rmA\mW],\text{diag}(\E[\mW^T\rmA\mW])\rangle\geq0$, we have
\begin{equation}
    \fn{\mM^*}\geq\fn{\E[\mW^T\rmA\mW]} = \fn{\mW^T\tilde{\rmA}\mW}.
\end{equation}
From equation \cref{lower-bound-c-1-eigenvalue-of-A}, we know that the first $(c-1)$ eigenvalues of $\tilde{\rmA}$ is bounded by some constant $\gamma\triangleq\beta^c\cdot\frac{\pr{\frac{\exp(-\alpha)}{c\exp(\alpha)}}^2}{2c}$ which is independent of $n$. Then we analyze the eigenvalues of $\mW^T\tilde{\rmA}\mW$: From \cref{lemma:WW-identity} and set $\eps=\frac12$, we know that the smallest singular value of $\mW$ is lower bounded by $\frac12$. Therefore, for any unit vector $v$ in the row span of $\mW$, we have
\begin{equation}
\label{eqn:WAW-lower-bound}
    v^T\mW^T\tilde{\rmA}\mW v = (\mW v)^T\tilde{\rmA}(\mW v) \geq \gamma\n{\mW v}^2 \geq \frac{\gamma}{4}.
\end{equation}
Thus, $\fn{\mW^T\tilde{\rmA}\mW}\geq\frac{\gamma}{4}$, which is some constant that is independent of $n$.

Besides, since $\rmD$ is a dignonal matrix with 0/1 entries, and the absolute value of each entry of $\rmA$ is bounded by 1, we have
\begin{equation}
    \fn{\mM}=\fn{\E[\rmD\mW^T\rmA\mW \rmD]}\leq\fn{\E[\mW^T\rmA\mW]}\leq\fns{\mW}\fn{\rmA}\leq c\fns{\mW}.
\end{equation}
From \cref{lemma:W-norm}, we know that with probability 1, $\fns{\mW}\leq 2c$, therefore, $\fn{\mM}$ is upper bounded by $2c^2$, which is independent of $n$.
\end{proofof}
Now we are ready to prove our main theorem.

%\\\textbf{Proof idea:} (Note: ``$A\approx B$'' means $\lim_{n\to\infty}\fns{A-B}=0$.)\\
%1. First, we know that $\fns{WMW^T}\approx\fns{M}$.\\
%2. Then, use $WW^T\approx I_c$ to show that $\fns{W^TWMW^TW}=\tr(W^TWMW^TWW^TWMW^TW)\approx \tr(W^TWW^TWMW^TW)=\tr(WW^TWMW^TWMW^T)\approx \tr(WMW^TWMW^T)=\fns{WMW^T}$.\\
%3. Therefore, $\fns{W^TWMW^TW}\approx\fns{M}$.
%Since the rows of $W$ are approximately unit norm and orthogonal, we know that $W^TW\approx P_W$, where $P_W$ is the orthogonal projection matrix projecting to row span of $W$, so $\fns{P_WMP_W}\approx\fns{M}$.\\
%4. Note that $\fns{M}=\fns{P_WMP_W}+\fns{P_WMP_W^\perp}+\fns{P_W^\perp MP_W}+\fns{P_W^\perp MP_W^\perp}$. From $\fns{P_WMP_W}\approx\fns{M}$ we know that $P_WMP_W^\perp, P_W^\perp MP_W, P_W^\perp MP_W^\perp\approx 0$. Since $M = P_WMP_W + P_WMP_W^\perp + P_W^\perp MP_W + P_W^\perp MP_W^\perp$, we conclude that $M\approx P_WMP_W\approx W^TWMW^TW$.\\
%5, From \cref{lemma:WMW-equivalence} we know that $WMW^T\approx WM^*W^T$, so $M\approx W^TWMW^TW\approx W^TWM^*W^TW\approx \frac14W^TAW$, for which we can analyze the eigenvalues and eigenspace using \cref{lemma:A-rank-c-1}.\\
%6. Use Davis-Kahan Theorem to bound the change of eigenvectors. The eigengap is the lower bound for $\lambda_{c-1}$ in \cref{lemma:A-rank-c-1}, and the Frob norm is the sum of all error terms caused by the``$\approx$'''s mentioned above.
%\\\\\textbf{Detailed proof:}
%
From \cref{corr:proj-preserve-F-norm} we have 
\begin{equation}
    \lim_{n\to\infty}\frac{\fns{\mW\mM\mW^T}}{\fns{\mM}}=1.
\end{equation}
Then we consider $\fns{\mW^T\mW\mM \mW^T\mW}$. Note that
\begin{equation}
\begin{split}
    \fns{\mW^T\mW\mM\mW^T\mW}&=\tr(\mW^T\mW\mM\mW^T\mW\mW^T\mW\mM\mW^T\mW)\\
    &=\tr(\mW\mW^T\mW\mM\mW^T\mW\mW^T\mW\mM\mW^T).
\end{split}
\end{equation}
From \cref{lemma:WW-identity} we know that for all $\eps'>0$, $\lim_{n\to\infty}\Pr(\n{\mW\mW^T-I_c}\geq\eps')=0$. For notation simplicity, in this proof we will omit the limit and probability arguments which can be dealt with using union bound. Therefore, we will directly state $\n{\mW\mW^T-I_c}\leq\eps'$. From \cite{kleinman1968design} we know that for positive semi-definite matrices $A$ and $B$ we have $\lambda_{\min}(A)\tr(B)\leq \tr(AB)\leq \lambda_{\max}(A)\tr(B)$, so
\begin{equation}\begin{split}
    &|\tr(\mW\mW^T\cdot \mW\mM \mW^T\mW\mW^T\mW\mM \mW^T) - \tr(\mW\mM \mW^T\mW\mW^T\mW\mM \mW^T)| \\
    \leq& \max\{1-\lambda_{\min}(\mW\mW^T), \lambda_{\max}(\mW\mW^T)-1\}\tr(\mW\mM \mW^T\mW\mW^T\mW\mM \mW^T)\\
    \leq& \n{\mW\mW^T-I_c}\tr(\mW\mM \mW^T\mW\mW^T\mW\mM \mW^T)\leq\eps'\tr(\mW\mM \mW^T\mW\mW^T\mW\mM \mW^T).
\end{split}
\end{equation}
Similarly,
\begin{equation}\begin{split}
    &|\tr(\mW\mM \mW^T\mW\mW^T\mW\mM \mW^T) - \tr(\mW\mM \mW^T\mW\mM \mW^T)|\\
    =&|\tr(\mW\mW^T\cdot \mW\mM \mW^T\mW\mM \mW^T) - \tr(\mW\mM \mW^T\mW\mM \mW^T)|\\
    \leq&\n{\mW\mW^T-I_c}\tr(\mW\mM \mW^T\mW\mM \mW^T)\leq\eps'\tr(\mW\mM \mW^T\mW\mM \mW^T).
\end{split}\end{equation}
Therefore,
\begin{equation}\begin{split}
    &|\fns{\mW^T\mW\mM \mW^T\mW}-\fns{\mW\mM \mW^T}|\\
    =&|\tr(\mW\mW^T\cdot \mW\mM \mW^T\mW\mW^T\mW\mM \mW^T) - \tr(\mW\mM \mW^T\mW\mM \mW^T)| \\
    \leq&|\tr(\mW\mW^T\cdot \mW\mM \mW^T\mW\mW^T\mW\mM \mW^T) - \tr(\mW\mM \mW^T\mW\mW^T\mW\mM \mW^T)|\\
    &+|\tr(\mW\mM \mW^T\mW\mW^T\mW\mM \mW^T) - \tr(\mW\mM \mW^T\mW\mM \mW^T)|\\
    \leq&\eps'\tr(\mW\mM \mW^T\mW\mW^T\mW\mM \mW^T)+\eps'\tr(\mW\mM \mW^T\mW\mM \mW^T)\\
    \leq&\eps'(1+\eps')\tr(\mW\mM \mW^T\mW\mM \mW^T)+\eps'\tr(\mW\mM \mW^T\mW\mM \mW^T)\\
    \leq&(2\eps'+(\eps')^2)\tr(\mW\mM \mW^T\mW\mM \mW^T) = (2\eps'+(\eps')^2)\fns{\mW\mM \mW^T}.
\end{split}\end{equation}
For all $\eps>0$, select $\eps'<\min\{\frac{\sqrt{\eps}}{2},\frac{\eps}{4}\}$, we have
\begin{equation}
    |\fns{\mW^T\mW\mM \mW^T\mW}-\fns{\mW\mM \mW^T}|<\eps \fns{\mW\mM \mW^T}.
\end{equation}
In other words,
\begin{equation}
    \lim_{n\to\infty}\frac{\fns{\mW^T\mW\mM \mW^T\mW}}{\fns{\mW\mM \mW^T}}=1.
\end{equation}
Hence we get
\begin{equation}
    \lim_{n\to\infty}\frac{\fns{\mW^T\mW\mM \mW^T\mW}}{\fns{\mM }}=1.
\end{equation}
Next, consider the orthogonal projection matrix $P_\mW$ that projects vectors in $R^n$ into the subspace spanned by all rows of $\mW$. We will consider the matrix $P_\mW\mM P_\mW$. Define $\delta\triangleq \mW^T\mW-P_\mW$, then from \cref{W-projection} we get $\fns{\delta}\leq\eps'$. Therefore,
\begin{equation}\begin{split}
    |\fn{\mW^T\mW\mM \mW^T\mW} - \fn{P_\mW\mM P_\mW}| &\leq \fn{P_\mW\mM \delta} + \fn{\delta \mM P_\mW} + \fn{\delta \mM \delta}\\
                                    &\leq \fn{\mM }\pr{2\fn{P_\mW}\fn{\delta}+\fns{\delta}}\\
                                    &\leq \fn{\mM }\pr{2\cdot 4c^2\eps'+(\eps')^2}.
\end{split}\end{equation}
For all $\eps>0$, we choose $\eps'<\min\{\frac{\sqrt{\eps}}{2},\frac{\eps}{16c^2}\}$ and have
\begin{equation}
    \frac{|\fn{\mW^T\mW\mM \mW^T\mW} - \fn{P_\mW\mM P_\mW}|}{\fn{\mM }} < \eps,
\end{equation}
which means that
\begin{equation}
    \lim_{n\to\infty}\frac{|\fn{\mW^T\mW\mM \mW^T\mW} - \fn{P_\mW\mM P_\mW}|}{\fn{\mW^T\mW\mM \mW^T\mW}}=\lim_{n\to\infty}\frac{|\fn{\mW^T\mW\mM \mW^T\mW} - \fn{P_\mW\mM P_\mW}|}{\fn{\mM }}=0.
\end{equation}
Thus,
\begin{equation}
    \lim_{n\to\infty}\frac{\fn{P_\mW\mM P_\mW}}{\fn{\mM }}=\lim_{n\to\infty}\frac{\fn{P_\mW\mM P_\mW}}{\fn{\mW^T\mW\mM \mW^T\mW}}=1.
\end{equation}
Note that $\fns{\mM }=\fns{P_\mW\mM P_\mW}+\fns{P_\mW\mM P_\mW^\perp}+\fns{P_\mW^\perp \mM P_\mW}+\fns{P_\mW^\perp \mM P_\mW^\perp}$. Therefore, 
\begin{equation}
    \lim_{n\to\infty}\frac{\fns{P_\mW\mM P_\mW^\perp}+\fns{P_\mW^\perp \mM P_\mW}+\fns{P_\mW^\perp \mM P_\mW^\perp}}{\fns{\mM }}=\lim_{n\to\infty}\frac{\fns{\mM }-\fns{P_\mW\mM P_\mW}}{\fns{\mM }}=0.
\end{equation}
In other words,
\begin{equation}
    \lim_{n\to\infty}\frac{\fn{P_\mW\mM P_\mW^\perp}}{\fn{\mM }}=\lim_{n\to\infty}\frac{\fn{P_\mW^\perp \mM P_\mW}}{\fn{\mM }}=\lim_{n\to\infty}\frac{\fn{P_\mW^\perp \mM P_\mW^\perp}}{\fn{\mM }}=0.
\end{equation}
From \cref{lemma:M-F-norm-bound} we know that $\lim_{n\to\infty}\fn{\mM }$ (this hasn't proved to be exist, so we perhaps need to say ``for large enough $n$'') is lower bounded by some constant that is independent of $n$, so
\begin{equation}
    \lim_{n\to\infty}\fn{P_\mW\mM P_\mW^\perp} = \lim_{n\to\infty}\fn{P_\mW^\perp \mM P_\mW} = \lim_{n\to\infty}\fn{P_\mW^\perp \mM P_\mW^\perp} = 0.
\end{equation}
Note that
\begin{equation}
    \mM  = P_\mW\mM P_\mW + P_\mW\mM P_\mW^\perp + P_\mW^\perp \mM P_\mW + P_\mW^\perp \mM P_\mW^\perp.
\end{equation}
Thus,
\begin{equation}
    \lim_{n\to\infty}\fn{\mM -P_\mW\mM P_\mW}=0.
\end{equation}
For any $\eps>0$, set $\delta<\min\{\frac{\eps\gamma}{8c^2},\frac{\sqrt{\eps\gamma}}{2c]}\}$, from \cref{W-projection}, we know that with probability 1, $\fn{P_\mW-\mW^T\mW}\leq\delta$. Therefore,
\begin{equation}\begin{split}
    &\fn{P_\mW\mM P_\mW-\mW^T\mW\mM \mW^T\mW}\\ \leq& \fns{P_\mW-\mW^T\mW}\fn{\mM } + 2\fn{P_\mW-\mW^T\mW}\fn{\mM }\fn{P_\mW}\\
                           \leq& \delta^2\cdot 2c^2 + 2\delta\cdot 2c^2\\
                           <& \eps.
\end{split}\end{equation}
In other words, 
\begin{equation}
    \lim_{n\to\infty}\fn{P_\mW\mM P_\mW-\mW^T\mW\mM \mW^T\mW}=0.
\end{equation}
Now we conclude that
\begin{equation}
    \lim_{n\to\infty}\fn{\mM -\mW^T\mW\mM \mW^T\mW} = 0.
\end{equation}
From \cref{lemma:WMW-equivalence} we know that $\forall i,j\in[c], \lim_{n\to\infty}((\mW\mM\mW^T)_{i,j}-(\mW\mM^*\mW^T)_{i,j})=0$, i.e.,
\begin{equation}
    \lim_{n\to\infty}\fn{\mW\mM \mW^T-\mW\mM^*\mW^T}=0.
\end{equation}
Since
\begin{equation}
    \fn{\mW^T\mW\mM \mW^T\mW-\mW^T\mW\mM^*\mW^T\mW}\leq \fns{\mW}\fn{\mW\mM \mW^T-\mW\mM^*\mW^T},
\end{equation}
from \cref{lemma:W-norm} which bounds the Frobenius norm of $\mW$ we know that
\begin{equation}
    \lim_{n\to\infty}\fn{\mW^T\mW\mM \mW^T\mW-\mW^T\mW\mM^*\mW^T\mW} = 0.
\end{equation}
Thus,
\begin{equation}
\label{eqn:M-equal-WTWMWTW}
    \lim_{n\to\infty}\fn{\mM-\mW^T\mW\mM^*\mW^T\mW} = 0.
\end{equation}
Note that $\mM^*=\frac14\left(\E[\mW^T\rmA\mW]+\text{diag}(\E[\mW^T\rmA\mW])\right)$, so
\begin{equation}
\label{eqn:M-approx-complex}
    4\mW^T\mW\mM^*\mW^T\mW = \mW^T\mW\mW^T\tilde{\rmA}\mW\mW^T\mW + \mW^T\mW\text{diag}(\E[\mW^T\rmA\mW])\mW^T\mW.
\end{equation}
We will first analyze the second term on the RHS of equation \cref{eqn:M-approx-complex}. $\forall\eps>0$, set $\eps'=\frac{\eps}{\sqrt{c}}$, and from \cref{lemma:WW-identity} we know that $\n{\mW\mW^T-I_c}<\eps'$ with probability 1, which means that $|\fn{\mW\mW^T}-c|<\eps$ with probability 1. Set $\eps=c$, we know that $\fn{\mW\mW^T}<2c$ with probability 1. Note that
\begin{equation}\begin{split}
    \fn{\mW^T\mW\text{diag}(\E[\mW^T\rmA\mW])\mW^T\mW} &\leq\fns{\mW^T\mW}\fn{\text{diag}(\E[\mW^T\rmA\mW])}\\
                                        &=\fns{\mW\mW^T}\fn{\text{diag}(\E[\mW^T\rmA\mW])}\\
                                        &\leq 4c^2\fn{\text{diag}(\E[\mW^T\rmA\mW])}.
\end{split}\end{equation}
Combine this with equation \cref{lemma:W-diag-neg} and we have
\begin{equation}
    \lim_{n\to\infty}\frac{\fn{\mW^T\mW\text{diag}(\E[\mW^T\rmA\mW])\mW^T\mW}}{\fn{\mW^T\tilde{\rmA}\mW}} = 0.
\end{equation}
From equation \cref{eqn:WAW-lower-bound} we know that $\fn{\mW^T\tilde{A}\mW}\geq\frac{\gamma}{4}$ with probability 1, so
\begin{equation}
\label{eqn:WTWMWTW-equal-WTWWTAWWTW}
    \lim_{n\to\infty}\fn{4\mW^T\mW\mM^*\mW^T\mW - \mW^T\mW\mW^T\tilde{\rmA}\mW\mW^T\mW} = 0.
\end{equation}
Similarly, define $\delta\triangleq \mW\mW^T-I_c$, then
\begin{equation}\begin{split}
    &\fn{\mW^T\mW\mW^T\tilde{\rmA}\mW\mW^T\mW - \mW^T\tilde{\rmA}\mW}\\
\leq&\fn{\mW^T\delta\tilde{\rmA}\delta \mW}+2\fn{\mW^T\tilde{\rmA}\delta}\\
\leq&\fns{\mW}\fns{\delta}\fn{\tilde{\rmA}} + 2\fn{\mW}\fn{\delta}\fn{\tilde{\rmA}}.
\end{split}\end{equation}
Set $\eps'<\min\{\frac{\eps}{8c^2},\sqrt{\frac{\eps}{8c^3}}\}$, then from \cref{lemma:WW-identity} we know that $\fn{\delta}<\eps'$ with probability 1, and from \cref{lemma:W-norm} we have $\fn{\mW}\leq 2c$ with probability 1. We also have $\fn{\tilde{\rmA}}\leq c$ since each entry of $\rmA$ is bounded by 1 in absolute value.
Therefore,
\begin{equation}
\fn{\mW^T\mW\mW^T\tilde{\rmA}\mW\mW^T\mW - \mW^T\tilde{\rmA}\mW} \leq 4c^2(\eps')^2\cdot c + 2\cdot 2c\eps'\cdot c < \frac{\eps}{2} + \frac{\eps}{2} = \eps,
\end{equation}
which means that
\begin{equation}
\label{eqn:WTWWTAWWTW-equal-WTAW}
    \lim_{n\to\infty}\fn{\mW^T\mW\mW^T\tilde{\rmA}\mW\mW^T\mW - \mW^T\tilde{\rmA}\mW} = 0.
\end{equation}
From equations \cref{eqn:M-equal-WTWMWTW}, \cref{eqn:WTWMWTW-equal-WTWWTAWWTW}, and \cref{eqn:WTWWTAWWTW-equal-WTAW} we get
\begin{equation}
    \lim_{n\to\infty}\fn{\mM - \frac14\mW^T\tilde{\rmA}\mW} = 0.
\end{equation}
Besides, from equation \cref{eqn:W-equal-W-bar} in \cref{W-projection} we know that for any $\eps'>0$,
\begin{equation}
    \fns{\overline{\mW}-\mW} = \sum_{i\in[c]} \ns{\overline{\mW}_i-\mW_i}<\eps',
\end{equation}
where $\overline{\mW}$ is the orthogonal version of $\mW$, i.e., we run the Gram-Schmidt process for the rows of $\mW$. Define $\delta\triangleq \overline{\mW}-\mW$, for any $\eps>0$, set $\eps'=\min\{\frac{\eps}{8c^2},\sqrt{\frac{\eps}{2c}}\}$, we have with probability 1,
\begin{equation}\begin{split}
    \fn{\mW^T\tilde{\rmA}\mW - \overline{\mW}^T\tilde{\rmA}\overline{\mW}} &\leq 2\fn{\delta}\fn{\tilde{\rmA}}\fn{\mW} + \fns{\delta}\fn{\tilde{\rmA}}\\
                                                             &4c^2\eps'+c(\eps')^2 < \eps.
\end{split}\end{equation}
Therefore,
\begin{equation}
    \lim_{n\to\infty}\fn{\mW^T\tilde{\rmA}\mW - \overline{\mW}^T\tilde{\rmA}\overline{\mW}} = 0,
\end{equation}
which implies
\begin{equation}
    \lim_{n\to\infty}\fn{\mM - \frac14\overline{\mW}^T\tilde{\rmA}\overline{\mW}} = 0.
\end{equation}
From \cref{lemma:A-rank-c-1} we know that with probability 1, $\tilde{\rmA}$ is of rank $(c-1)$. Since $\rmA\cdot\textbf{1}=0$ is always true, the top $(c-1)$ eigenspace of $\tilde{\rmA}$ is $\R^c\backslash\{\textbf{1}\}$. Note that the rows in $\overline{\mW}$ are of unit norm and orthogonal to each other, we conclude that $\overline{\mW}^T\tilde{\rmA}\overline{\mW}$ is of rank $(c-1)$ and the corresponding eigenspace is $\gR\{\overline{\mW}_i\}_{i=1}^c\backslash\{\overline{\mW}\cdot\textbf{1}\}$. Moreover, the minimum positive eigenvalue of $\overline{\mW}^T\tilde{\rmA}\overline{\mW}$ is lower bounded by $\gamma$.

As for the top $c-1$ eigenvectors of $\mM$, define $\delta\triangleq\mM-\frac14\overline{\mW}^T\tilde{\rmA}\overline{\mW}$, then $\mM = \frac14\overline{\mW}^T\tilde{\rmA}\overline{\mW} + \delta$. Define $S_1$ as the top $c-1$ eigenspaces for $\mM$, and $S_2$ to be the top $c-1$ eigenspaces for $\frac14\overline{\mW}^T\tilde{\rmA}\overline{\mW}$. Then from Davis-Kahan Theorem we know that
\begin{equation}
    \fn{\sin\Theta(S_1,S_2)}\leq\frac{\fn{\delta}}{\lambda_{c-1}(\frac14\overline{\mW}^T\tilde{\rmA}\overline{\mW})}.
\end{equation}
Here $\Theta(S_1,S_2)$ is a $(c-1)\times(c-1)$ diagonal matrix whose $i$-th diagonal entry is the $i$-th canonical angle between $S_1$ and $S_2$. Since $\lim_{n\to\infty}\fn{\delta}=0$, and with probability 1, $\lambda_{c-1}(\frac14\overline{\mW}^T\tilde{\rmA}\overline{\mW})\geq\gamma$ which is independent of $n$, we have with probability 1,
\begin{equation}
    \lim_{n\to\infty}\fn{\sin\Theta(S_1,S_2)} = 0,
\end{equation}
which indicates that the top $c-1$ eigenspaces for $\mM$ and $\frac14\overline{\mW}^T\tilde{\rmA}\overline{\mW}$ are the same when $n\to\infty$.

Notice that the top $c-1$ eigenspaces of $\overline{\mW}^T\tilde{\rmA}\overline{\mW}$ are $\gR\{\overline{\mW}_i\}_{i=1}^c\backslash\{\overline{\mW}\cdot\textbf{1}\}$, so $\mM$ will also have the same top $c-1$ eigenspaces. Besides, from equation \cref{eqn:W-equal-W-bar} we know that $\lim_{n\to\infty}\fn{\mW-\overline{\mW}}=0$, so $\gR\{\overline{\mW}_i\}_{i=1}^c\backslash\{\overline{\mW}\cdot\textbf{1}\}$ are the same as $\gR\{\mW_i\}_{i=1}^c\backslash\{\mW\cdot\textbf{1}\}$. This completes the proof of this theorem.

\end{proofof}

\subsection{Experiment Results}
\input{Appendix_Sections/Output_Hessian_Proof/output_hessian_exp_result}

%\end{document} 

\section{Codes Description}
\label{sec:app_codes}
%We include 3 packages in the source codes: \emph{closeformhessian}, \emph{hessian\_eigenthings}, and \emph{eigen\_pac\_bayes}.

%\emph{closeformhessian} gives the methods to calculate matrices we used in our experiments, like $\E[\mM]$ and $\E[\vx\vx^T]$, and others mentioned in \cref{sec:appendix_derivation_main}. Most of the computational functions are in decomp.py. The names should be self-explanatory, except that we use some old namings (U for $\mG$, UTAU for $\mM$).

%\emph{hessian\_eigenthings} is used to calculate eigenvalues and eigenvectors as described in \cref{sec:appendix_eigencomp}, modified from \citet{hessian-eigenthings}. 

The complete set of experiment code for this paper are included in the folder \textbf{Dissecting\_Hessian\_Codebase} of the supplemental material.

All of our experiment code are are based on Python and PyTorch \citep{NEURIPS2019_9015}. The README file in the code base folder provides a brief introduction to the structure of the code base along with required environments.
