# Supplementary material for: Dissecting Hessian: Understanding Common Structure of Hessian in Neural Networks
Source: arXiv:2010.04261 source file (2022-10-21)
Supplement: Supplementary file 3 [file codes.tex]

\label{sec:app_codes}
%We include 3 packages in the source codes: \emph{closeformhessian}, \emph{hessian\_eigenthings}, and \emph{eigen\_pac\_bayes}.

%\emph{closeformhessian} gives the methods to calculate matrices we used in our experiments, like $\E[\mM]$ and $\E[\vx\vx^T]$, and others mentioned in \cref{sec:appendix_derivation_main}. Most of the computational functions are in decomp.py. The names should be self-explanatory, except that we use some old namings (U for $\mG$, UTAU for $\mM$).

%\emph{hessian\_eigenthings} is used to calculate eigenvalues and eigenvectors as described in \cref{sec:appendix_eigencomp}, modified from \citet{hessian-eigenthings}. 

The complete set of experiment code for this paper are included in the folder \textbf{Dissecting\_Hessian\_Codebase} of the supplemental material.

All of our experiment code are are based on Python and PyTorch \citep{NEURIPS2019_9015}. The README file in the code base folder provides a brief introduction to the structure of the code base along with required environments.
